# Supplementary material for: Going Beyond Linear RL: Sample Efficient Neural Function Approximation
Source: arXiv:2107.06466 source file (2021-12-25)
Supplement: Supplementary file 1 [file appendix.pdf]

---

# Going Beyond Linear RL: Sample Efficient Neural Function Approximation

---

Anonymous Author(s)

Affiliation

Address

email

## Abstract

1        Deep Reinforcement Learning (RL) powered by neural net approximation of the  
2        Q function has had enormous empirical success. While the theory of RL has  
3        traditionally focused on linear function approximation (or eluder dimension) ap-  
4        proaches, little is known about nonlinear RL with neural net approximations of the  
5        Q functions. This is the focus of this work, where we study function approximation  
6        with two-layer neural networks (considering both ReLU and polynomial activation  
7        functions). Our first result is a computationally and statistically efficient algorithm  
8        in the generative model setting under completeness for two-layer neural networks.  
9        Our second result considers this setting but under only realizability of the neural  
10       net function class. Here, assuming deterministic dynamics, the sample complexity  
11       scales linearly in the algebraic dimension. In all cases, our results significantly  
12       improve upon what can be attained with linear (or eluder dimension) methods.

## 13    1 Introduction

14    In reinforcement learning (RL), an agent aims to learn the optimal decision-making rule by interacting  
15    with unknown environment [Sutton and Barto, 2018]. Deep Reinforcement Learning, empowered  
16    by deep neural networks [LeCun et al., 2015, Goodfellow et al., 2016], has achieved tremendous  
17    success in various real-world applications, such as Go [Silver et al., 2016], Atari [Mnih et al., 2013a],  
18    Dota2 [Berner et al., 2019], Texas Holdém poker [Moravčík et al., 2017], and autonomous driving  
19    [Shalev-Shwartz et al., 2016]. Those modern RL applications are characterized by large state-action  
20    spaces, and the empirical success of deep RL corroborates the observation that deep neural networks  
21    can extrapolate well across state-action spaces [Henderson et al., 2018, Mnih et al., 2013b, Lillicrap  
22    et al., 2015].

23    Although in practice non-linear function approximation scheme is prevalent, theoretical understand-  
24    ings of the sample complexity of RL mainly focus on tabular or linear function approximation  
25    settings [Strehl et al., 2006, Jaksch et al., 2010, Azar et al., 2017, Jin et al., 2018, Russo, 2019,  
26    Zanette and Brunskill, 2019, Abbasi-Yadkori et al., 2019, Jin et al., 2020a,b, Wang et al., 2021a].  
27    These results rely on finite state space or exact linear approximations. Recently, sample efficient  
28    algorithms under non-linear function approximation settings are proposed [Wen and Van Roy, 2017,  
29    Dann et al., 2018, Du et al., 2019b, Dong et al., 2020, Liu et al., 2019, Wang et al., 2020a, Dong  
30    et al., 2021]. Those algorithms are based on Bellman rank [Jiang et al., 2017], eluder dimension  
31    [Russo and Van Roy, 2013b], neural tangent kernel [Jacot et al., 2018, Allen-Zhu et al., 2019, Du  
32    et al., 2019a], or sequential Rademacher complexity [Rakhlin et al., 2015a,b]. Besides, general neural  
33    network function approximation is shown to be hard by Dong et al. [2021]. Yet, there is a mismatch

34 between the empirical success of deep RL and the theoretical understanding of RL under general  
 35 deep neural network function approximations, which yields the following important question:

36 *What are the structural properties that allow sample-efficient algorithms for RL with neural network*  
 37 *function approximation?*

38 In this paper, we advance our understanding to the above question by considering several settings  
 39 where structural reconstruction can be achieved. Specifically, we study two structures, namely two-  
 40 layer neural networks and structured polynomials, under two RL settings, namely RL with simulator  
 41 model and online RL. In the simulator (generative model) setting [Kakade, 2003, Sidford et al., 2018],  
 42 the agent can simulate the MDP at any state-action pair. In online RL, the agent can only start at an  
 43 initial state and interact with the MDP step-by-step. Our goal is to find near-optimal policy while  
 44 minimizing the number of samples used.

45 We obtain the following results. For the simulator setting, we propose sample-efficient algorithms  
 46 for RL with two-layer neural network function approximation, under the Bellman completeness  
 47 assumption. For online RL, we provide sample-efficient algorithms for RL with structured polynomial  
 48 function approximation. We also present sample-efficient algorithms under realizability assumption  
 49 [Du et al., 2020b, Wang et al., 2021b], but with deterministic transition. Our main techniques are  
 50 neural network recovery [Zhong et al., 2017], and algebraic geometry [Shafarevich, 2013].

## 51 1.1 Summary of our results

52 Our main results in different settings are summarized in Table 1. We consider two-layer neural  
 networks  $f(x) = \langle v, \sigma(Wx) \rangle$  and rank  $k$  polynomials (see Example 5.3). We make the following

Table 1: Baselines and our main results for the sample complexity to find a  $\epsilon$ -optimal policy.

|             | rank $k$ polynomial |                   | Neural Net of Width $k$              |                                   |
|-------------|---------------------|-------------------|--------------------------------------|-----------------------------------|
|             | Sim. + Det. (R)     | Online + Det. (R) | Sim. + Det. (R)                      | Sim. + Stoch. (C)                 |
| Baseline    | $O(d^p)$            | $O(d^p)$          | $O(d^{\text{poly}(1/\epsilon)})$ (*) | $O(d^{\text{poly}(1/\epsilon)})$  |
| Our results | $O(dk)$             | $O(dk)$           | $O(\text{poly}(d) \exp(k))$          | $O(\text{poly}(d, k)/\epsilon^2)$ |

53  
 54 elaborations on Table 1.

- 55 • We show the dependence on the feature dimension  $d$ , network width or polynomial rank  $k$ ,  
 56 precision  $\epsilon$ , and degree  $p$ .
- 57 • For the setting: Sim. denotes simulator model, Online denotes online RL, Det. denotes  
 58 deterministic transitions, Stoch. denotes stochastic transitions, (R) denotes realizability  
 59 assumption only, and (C) denotes completeness assumption.
- 60 • For the deterministic transition baseline, we apply Du et al. [2020c] and for the stochastic  
 61 transition baseline we apply Du et al. [2020a]. We are unaware of any methods that can  
 62 directly learn MDP with neural network value function approximation<sup>1</sup>.
- 63 • In polynomial case, the baseline first vectorizes the tensor  $\begin{pmatrix} 1 \\ x \end{pmatrix}^{\otimes p}$  into a vector in  $\mathbb{R}^{(d+1)^p}$   
 64 and then performs on this vector. In the neural network case, the baseline uses a polynomial  
 65 of degree  $1/\epsilon$  to approximate the neural network with precision  $\epsilon$  and then vectorizes the  
 66 polynomial into a vector in  $\mathbb{R}^{d^{\text{poly}(1/\epsilon)}}$ . The baseline method for realizable model (denoted  
 67 by (\*)) needs a further gap assumption of  $\text{gap} \geq d^{\text{poly}(1/\epsilon)} \epsilon$  to avoid the approximation  
 68 error from propagating Du et al. [2020c]; note for small  $\epsilon$  this condition never holds but we  
 69 include it in the table for the sake of comparison.
- 70 • In rank  $k$  polynomial case, our result  $O(dk)$  in simulator model can be found in Theorem 5.7  
 71 and our result  $O(dk)$  in online RL model can be found in Theorem 5.8. These results only  
 72 require realizability assumption. Efficient explorations are guaranteed by algebraic geometric  
 73 arguments. In neural network model, our result  $O(\text{poly}(d) \exp(k))$  in simulator model can

be found in Theorem 4.4. This result also only relies on the realizability assumption. For stochastic transitions, our result  $O(\text{poly}(d, k)/\epsilon^2)$  works for both policy complete and Bellman complete setting, as in Theorem 4.5 and Theorem 4.6 respectively.

## 2 Related Works

**Linear Function Approximation.** RL with linear function approximation has been widely studied under various settings, including linear MDP and linear mixture MDP [Jin et al., 2020b, Zanette et al., 2020, Yang and Wang, 2020]. While these papers have proved efficient regret and sample complexity bounds, their analyses relied heavily on two techniques: they used the confidence ellipsoid to quantify the uncertainty, and they used the elliptical potential lemma to bound the cumulative amount of uncertainty [Abbasi-Yadkori et al., 2011]. These two techniques were integral to their analyses, but were so restrictive that they could hardly be extended to nonlinear cases.

**Eluder Dimension.** Russo and Van Roy [2013a], Osband et al. [2013] came up with the notion of eluder dimension, which served as a complexity measure of the function space. In addition, they proved regret and sample complexity bounds that scaled with the eluder dimension, and showed that the eluder dimension is small (i.e. not exponentially large) in several settings, including generalized linear models and LQR. Wang et al. [2020b], Jin et al. [2021] extend Eluder dimension to reinforcement learning. However, as shown in [Dong et al., 2021], the eluder dimension could be exponentially large even with a single ReLU neuron, which suggested eluder dimension would face difficulty in dealing with neural network cases.

**Bellman Rank and Completeness.** Jiang et al. [2017], Sun et al. [2019] studied RL with general function approximation. They used Bellman rank to measure the error of the function class under the Bellman operator, and gave proved bounds in the term of it. Recently, Du et al. [2021] propose Bilinear rank and encompass more function approximation models. However, it is hard to bound the Bellman rank or Bilinear rank for neural nets, so their results are not known to include the neural network approximation setting. Another line of work (Du et al. [2020a], Weisz et al. [2020], Wang et al. [2021b]) shows that exponential sample complexity is unavoidable even with good representations.

## 3 Preliminaries

An episodic Markov Decision Process (MDP) is defined by the tuple  $\mathcal{M} = (\mathcal{S}, \mathcal{A}, H, \mathbb{P}, r)$  where  $\mathcal{S}$  is the state space,  $\mathcal{A}$  is the action set,  $H$  is the number of time steps in each episode,  $\mathbb{P}$  is the transition kernel and  $r$  is the reward function. In each episode the agent starts at a fixed initial state  $s_1$  and at each time step  $h \in [H]$  it takes action  $a_h$ , receives reward  $r_h(s_h, a_h)$  and transits to  $s_{h+1} \sim \mathbb{P}(\cdot | s_h, a_h)$ .

A deterministic policy  $\pi$  is a length- $H$  sequence of functions  $\pi = \{\pi_h : \mathcal{S} \mapsto \mathcal{A}\}_{h=1}^H$ . Given a policy  $\pi$ , we define the value function  $V_h^\pi(s)$  as the expected sum of reward under policy  $\pi$  starting from  $s_h = s$ :

$$V_h^\pi(s) := \mathbb{E} \left[ \sum_{t=h}^H r_t(s_t, a_t) | s_h = s \right]$$

and we define the Q function  $Q_h^\pi(s, a)$  as the the expected sum of reward taking action  $a$  in state  $s_h = s$  and then following  $\pi$ :

$$Q_h^\pi(s, a) := \mathbb{E} \left[ \sum_{t=h}^H r_t(s_t, a_t) | s_h = s, a_h = a \right].$$

---

<sup>1</sup>Prior work on neural function approximation has focused on neural tangent kernels, which would require  $d^{\text{poly}(1/\epsilon)}$  to approximate a two-layer network Ghorbani et al. [2021].

112 The Bellman operator  $\mathcal{T}_h$  applied to Q-function  $Q_{h+1}$  is defined as follow

$$\mathcal{T}_h(Q_{h+1})(s, a) := r_h(s, a) + \mathbb{E}_{s' \sim \mathbb{P}(\cdot|s, a)}[\max_{a'} Q_{h+1}(s', a')].$$

113 There exists an optimal policy  $\pi^*$  that gives the optimal value function for all states, i.e.  $V_h^{\pi^*}(s) =$   
 114  $\sup_{\pi} V_h^{\pi}(s)$  for all  $h \in [H]$  and  $s \in \mathcal{S}$ . For notational simplicity we abbreviate  $V^{\pi^*}$  as  $V^*$  and  
 115 correspondingly  $Q^{\pi^*}$  as  $Q^*$ . Therefore  $Q^*$  satisfies the following Bellman optimality equations for  
 116 all  $s \in \mathcal{S}$ ,  $a \in \mathcal{A}$  and  $h \in [H]$ :

$$Q_h^*(s, a) = \mathcal{T}_h(Q_{h+1}^*)(s, a).$$

117 The goal is to find a policy  $\pi$  that is  $\epsilon$ -optimal in the sense that  $V_1^*(s_1) - V_1^{\pi}(s_1) \leq \epsilon$ , within a small  
 118 number of samples. We consider two query models of interacting with MDP:

- 119 • In the simulator model (Kakade [2003], Sidford et al. [2018]), the agent interacts with  
 120 a black-box that simulates the MDP. At each time step  $h \in [H]$ , the agent can start at a  
 121 state-action pair  $(s, a)$  and interact with the black box by executing some policy  $\pi$  chosen  
 122 by the agent.
- 123 • In online RL, the agent can only start at the initial state and interact with the MDP by using  
 124 a policy and observing the rewards and the next states. In each episode  $k$ , the agent proposes  
 125 a policy  $\pi^k$  based on all history up to episode  $k - 1$  and executes  $\pi^k$  to generate a single  
 126 trajectory  $\{s_h^k, a_h^k\}_{h=1}^H$  with  $a_h^k = \pi_h^k(s_h^k)$  and  $s_{h+1}^k \sim \mathbb{P}_h(\cdot|s_h^k, a_h^k)$ .

### 127 3.1 Function approximation

128 In reinforcement learning with value function approximation, the learner is given a function class  
 129  $\mathcal{F} = \mathcal{F}_1 \times \dots \times \mathcal{F}_H$ , where  $\mathcal{F}_h \subset \{f : \mathcal{S} \times \mathcal{A} \mapsto [0, 1]\}$  is a set of candidate functions to approximate  
 130  $Q^*$ . The following assumption is commonly adopted in the literature.

131 **Assumption 3.1** (Realizability).  $Q_h^* \in \mathcal{F}_h$  for all  $h \in [H]$ .

132 The function approximation is equipped with feature mapping  $\phi : \mathcal{S} \times \mathcal{A} \mapsto \{u \in \mathbb{R}^d : \|u\|_2 \leq$   
 133  $B_{\phi}\}$  that is known to the agent. We make the following assumption about  $\phi$  that allows efficient  
 134 explorations.

135 **Assumption 3.2** (Dense features). We assume the image of  $\phi$  contains the ball  $\{u \in \mathbb{R}^d : \|u\|_2 \leq$   
 136  $d \text{polylog}(d)\}$ .

137 **Notation** For any vector  $x \in \mathbb{R}^d$ , let  $x_{\max} := \max_{i \in [d]} x_i$  and  $x_{\min} := \min_{i \in [d]} x_i$ . Let  $s_i(\cdot)$   
 138 denote the  $i$ -th singular value,  $s_{\min}(\cdot)$  denotes the minimum eigenvalue and  $s_{\max}(\cdot)$  denotes the  
 139 maximum eigenvalue. The conditional number is defined by  $\kappa(\cdot) := s_{\max}(\cdot)/s_{\min}(\cdot)$ . We use  $\otimes$  to  
 140 denote Kronecker product and  $\circ$  to denote Hadamard product. For a given integer  $H$ , we use  $[H]$  to  
 141 denote the set  $\{1, 2, \dots, H\}$ .

## 142 4 Neural Network Function Approximation

143 In this section we show sample efficient algorithms with neural network function approximations.  
 144 The function class of interest is given in the following definition. More general neural network class  
 145 is discussed in Section 4.

146 **Definition 4.1** (Neural Network Function Class). We use  $\mathcal{F}_{NN}$  to denote the function class of  
 147  $f(\phi(s, a)) : \mathcal{S} \times \mathcal{A} \mapsto \mathbb{R}$  where  $f(x) = \langle v, \sigma(Wx) \rangle$  is a two-layer neural network where  $\sigma$  is ReLU,  
 148  $\|W\|_F \leq B_W$ ,  $\prod_{i=1}^k s_i(W)/s_{\min}(W) \leq \lambda$ ,  $s_{\max}(W)/s_{\min}(W) \leq \kappa$  and  $k \leq d$ .

149 We introduce the following completeness properties in the setting of value function approximations.  
 150 Along with Assumption 3.1, they are commonly adopted in the literature.

151 **Definition 4.2** (Policy complete). Given MDP  $\mathcal{M} = (\mathcal{S}, \mathcal{A}, \mathbb{P}, r, H)$ , function class  $\mathcal{F}_h : \mathcal{S} \times \mathcal{A} \mapsto$   
 152  $\mathbb{R}$ ,  $h \in [H]$  is called policy complete iff for all  $\pi$  and  $h \in [H]$ ,  $Q_h^{\pi} \in \mathcal{F}_h$ .

153 **Definition 4.3** (Bellman complete). Given MDP  $\mathcal{M} = (\mathcal{S}, \mathcal{A}, \mathbb{P}, r, H)$ , function class  $\mathcal{F}_h : \mathcal{S} \times \mathcal{A} \mapsto$   
 154  $\mathbb{R}$ ,  $h \in [H]$  is called Bellman complete iff for all  $h \in [H]$  and  $Q_{h+1} \in \mathcal{F}_{h+1}$ ,  $\mathcal{T}_h(Q_{h+1}) \in \mathcal{F}_h$ .

#### 155 4.1 Warmup: Realizable $Q^*$ with deterministic transition

156 We start by considering the setting that transition kernel is deterministic. In this case only Assump-  
 157 tion 3.1 is required for neural network function approximations. The learning procedure, presented in  
 158 Algorithm 1, learns optimal policy from time step  $H$  to 1. Suppose we have learned optimal policy  
 159  $\pi_{h+1}, \dots, \pi_H$  at level  $h$ , we can then query features from a standard Gaussian distribution and if  
 160  $\|\phi(s, a)\|_2 \geq B_\phi$  then it simply skips this trial. Notice that  $B_\phi \geq d^2$ , so with high probability <sup>2</sup> most  
 161 samples fall in the feature set  $\{u \in \mathbb{R}^d : \|u\|_2 \leq B_\phi\}$ . We next construct an estimate  $\hat{Q}_h$  of  $Q^*$  by  
 162 using  $\pi_{h+1}, \dots, \pi_H$  as the roll-out. Since the transition is deterministic,  $\hat{Q}_h(s_h^i, a_h^i) = Q^*(s_h^i, a_h^i)$   
 163 and for all the samples  $\{(s_h^i, a_h^i) : i \in [n]\}$ . Recall  $Q_h^*$  is a two-layer neural network, we can now  
 164 recover its parameters in Step 8 exactly by invoking techniques in neural network optimization (see,  
 165 e.g. Janzamin et al. [2015], Ge et al. [2017], Zhong et al. [2017]). Details of this step can be found in  
 166 Appendix A.4. Making using of exact recovery of  $Q_h^*$ , the algorithm can thus find optimal policy  $\pi_h^*$ .

---

#### Algorithm 1 Learning realizable $Q^*$ with deterministic transition

---

```

1: for  $h = H, \dots, 1$  do
2:   Sample  $\phi(s_h^i, a_h^i), i \in [n]$  from standard Gaussian  $N(0, I_d)$ 
3:    $\triangleright$  If  $\|\phi(s_h^i, a_h^i)\|_2 \geq B_\phi$  then skip this trial.
4:   for  $i \in [n]$  do
5:     Query  $(s_h^i, a_h^i)$  and use  $\pi_{h+1}, \dots, \pi_H$  as the roll-out to collect rewards  $r_h^{(i)}, \dots, r_H^{(i)}$ 
6:     Construct estimation
           
$$\hat{Q}_h^{\pi_{h+1}, \dots, \pi_H}(s_h^i, a_h^i) = r_h^{(i)} + \dots + r_H^{(i)}$$

7:   end for
8:   Recover  $v_h$  and  $W_h$  from samples  $\{\phi(s_h^i, a_h^i), \hat{Q}_h^{\pi_{h+1}, \dots, \pi_H}(s_h^i, a_h^i) : i \in [n]\}$  using method
     of moments and gradient descent.
9:   Set  $\hat{Q}_h(s, a) \leftarrow v_h^\top \sigma(W_h \phi(s, a))$ 
10:  Set  $\pi_h(s) \leftarrow \arg \max_{a \in \mathcal{A}} \hat{Q}_h(s, a)$ 
11: end for
12: Return  $\pi_1, \dots, \pi_H$ 

```

---

167 **Theorem 4.4.** Suppose sample complexity  $n \geq d \cdot \text{poly}(\kappa, k, \lambda, \log d, B_W, B_\phi, H)$ , then with high  
 168 probability Algorithm 2 learns optimal policy  $\pi^*$ .

169 The complete proof is deferred to Appendix. The main idea of exact neural network recovery can be  
 170 summarized in the following. We first use method of moments to find a ‘rough’ parameter recovery.  
 171 If this ‘rough’ recovery is sufficiently close to the true parameter, the loss function is locally strongly  
 172 convex and there is unique global minimum. Then we can apply gradient descent to find this global  
 173 minimum which is exactly the true parameter.

#### 174 4.2 Policy complete neural function approximation

175 Now we consider general stochastic transitions. Difficulty arises in this scenario due to noises  
 176 in the estimation of Q-functions. In the presence of model misspecification, these noises cause  
 177 estimation errors to amplify through levels and require samples to be exponential in  $H$ . In this  
 178 section we show that neural network function approximation is still learnable assuming the function  
 179 class  $\mathcal{F}_{NN}$  is policy complete with regard to MDP  $\mathcal{M}$ . Thus for all  $\pi \in \Pi$ , we can denote  
 180  $Q_h^\pi(s, a) = \langle v^\pi, \sigma(W^\pi \phi(s, a)) \rangle$ .

181 Algorithm 2 learns policy from level  $H, H-1, \dots, 1$ . In level  $h$ , the algorithm has learned policy  
 182  $\pi_{h+1}, \dots, \pi_H$  that is only sub-optimal by  $(H-h)\epsilon/H$ . Then it selects features  $\phi(s, a)$  from  $\mathcal{N}(0, I_d)$ .

---

<sup>2</sup>Here with high probability is with respect to  $d$ .

---

**Algorithm 2** Learn policy complete NN with simulator.

---

```

1: Input: Precision  $\epsilon$ .
2: for  $h = H, \dots, 1$  do
3:   Sample  $\phi(s_h^i, a_h^i), i \in [n]$  from standard Gaussian  $N(0, I_d)$ 
4:    $\triangleright$  If  $\|\phi(s_h^i, a_h^i)\|_2 \geq B_\phi$  then skip this trial.
5:   for  $i \in [n]$  do
6:     Query  $(s_h^i, a_h^i)$  and use  $\pi_{h+1}, \dots, \pi_H$  as the roll-out to collect rewards  $r_h^{(i)}, \dots, r_H^{(i)}$ 
7:     Construct unbiased estimation
           
$$\widehat{Q}_h^{\pi_{h+1}, \dots, \pi_H}(s_h^i, a_h^i) = r_h^{(i)} + \dots + r_H^{(i)}$$

8:   end for
9:   Retrieve  $v_h$  and  $W_h$  from samples  $\{\phi(s_h^i, a_h^i), \widehat{Q}_h^{\pi_{h+1}, \dots, \pi_H}(s_h^i, a_h^i) : i \in [n]\}$ 
10:  Set  $\widehat{Q}_h(s, a) \leftarrow v_h^\top \sigma(W_h \phi(s, a))$ 
11:  Set  $\pi_h(s) \leftarrow \arg \max_{a \in \mathcal{S}} \widehat{Q}_h(s, a)$ 
12: end for
13: Return  $\pi_1, \dots, \pi_H$ 

```

---

183 The algorithm then queries  $(s, a)$  and uses learned policy  $\pi_{h+1}, \dots, \pi_H$  as roll out to collect an  
184 unbiased estimate of Q-function  $\widehat{Q}_h^{\pi_{h+1}, \dots, \pi_H}(s, a)$ . Recall that  $Q_h^{\pi_{h+1}, \dots, \pi_H}(s, a) \in \mathcal{F}_{NN}$  is a two-  
185 layer neural network, it can then be recovered from estimates. Details of this step can be found in  
186 Appendix A.4. The algorithm then finds optimal policy  $\pi_h$  and proceed to the level  $h - 1$ .

187 **Theorem 4.5.** Suppose sample complexity  $n \geq \epsilon^{-2} \cdot d \cdot \text{poly}(\kappa, k, \log d, B_W, B_\phi, H)$ , then with  
188 high probability Algorithm 2 learns an  $\epsilon$ -optimal policy  $\pi$ .

189 The sample complexity does not depend on  $\lambda$ , unlike the case of Theorem 4.4.

190 The main idea of the proof is that at each time step a neural network surrogate of  $Q^*$  can be constructed  
191 by the policy already learned. Suppose we have learned  $\pi_{h+1}, \dots, \pi_H$  in level  $h$ , then from policy  
192 completeness  $Q_h^{\pi_{h+1}, \dots, \pi_H}$  belongs to  $\mathcal{F}_{NN}$  and we can interact with the simulator to obtain its  
193 estimate  $\widehat{Q}_h$ . If  $\|\widehat{Q}_h - Q_h^{\pi_{h+1}, \dots, \pi_H}\|_\infty$  is small, the optimistic planning based on  $\widehat{Q}_h$  is not far from  
194 the optimal policy of  $Q_h^{\pi_{h+1}, \dots, \pi_H}$ . This reasoning can then be performed to level  $h - 1$ . The full  
195 proof of Theorem 4.5 is deferred to Section A.2.

### 196 4.3 Bellman complete neural function approximation

197 In addition to policy completeness, we show that neural network function approximation can also  
198 learn efficiently under the setting where the function class  $\mathcal{F}_{NN}$  is Bellman complete with regard to  
199 MDP  $\mathcal{M}$ . Specifically, for  $Q_{h+1} \in \mathcal{F}_{h+1}$ , there are  $v^{Q_{h+1}}$  and  $W^{Q_{h+1}}$  such that  $\mathcal{T}_h(Q_{h+1})(s, a) =$   
200  $\langle v^{Q_{h+1}}, \sigma(W^{Q_{h+1}} \phi(s, a)) \rangle$ .

201 Algorithm 3 is similar to the algorithm in previous section. In level  $h$ , the algorithm has constructed  
202 the Q-function  $\widehat{Q}_{h+1}(s, a) = v_{h+1}^\top \sigma(W_{h+1} \phi(s, a))$  that is  $(H - h)\epsilon/H$ -close to the optimal  $Q_{h+1}^*$ .  
203 It then recovers weights  $v_h, W_h$  from  $\mathcal{T}_h(\widehat{Q}_{h+1})(s, a) = \langle v^{\widehat{Q}_{h+1}}, \sigma(W^{\widehat{Q}_{h+1}} \phi(s, a)) \rangle$ , using unbiased  
204 estimates  $r_h(s_h^i, a_h^i) + \widehat{V}_{h+1}(s_{h+1}^i)$  for all  $i \in [n]$ . Details of this step can be found in Appendix A.4.  
205 The Q-function  $\widehat{Q}_h(s, a) = v_h^\top \sigma(W_h \phi(s, a))$  constructed from weights  $v_h, W_h$  is thus  $(H - h +$   
206  $1)\epsilon/H$ -close to the optimal  $Q_h^*$ .

207 **Theorem 4.6.** Suppose sample complexity  $n \geq \epsilon^{-2} \cdot d \cdot \text{poly}(\kappa, k, \log d, B_W, B_\phi, H)$ , then with  
208 high probability Algorithm 3 learns an  $\epsilon$ -optimal policy  $\pi$ .

209 Similar to Theorem 4.5, the sample complexity does not explicitly depend on  $\lambda$ .

210 Due to Bellman completeness, the error of estimation  $\widehat{Q}_h$  can be controlled recursively. In fact, we  
211 can show  $\|\widehat{Q}_h - Q^*(s, a)\|_\infty$  is small by induction. The full proof of Theorem 4.6 is deferred to  
212 Section A.3.

---

**Algorithm 3** Learn Bellman complete NN with simulator.

---

```

1: Input: Precision  $\epsilon$ .
2: for  $h = H, \dots, 1$  do
3:   Sample  $\phi(s_h^i, a_h^i), i \in [n]$  from standard Gaussian  $N(0, I_d)$ 
4:    $\triangleright$  If  $\|\phi(s_h^i, a_h^i)\|_2 \geq B_\phi$  then skip this trial.
5:   for  $i \in [n]$  do
6:     Query  $(s_h^i, a_h^i)$  and observe  $r_h(s_h^i, a_h^i), s_{h+1}^i$ 
7:   end for
8:   Retrieve  $v_h$  and  $W_h$  from  $\{\phi(s_h^i, a_h^i), r_h(s_h^i, a_h^i) + \hat{V}_{h+1}(s_{h+1}^i) : i \in [n]\}$ 
9:   Set  $\hat{Q}_h(s, a) \leftarrow v_h^\top \sigma(W_h \phi(s, a))$  and  $\hat{V}_h \leftarrow \max_{a \in \mathcal{A}} \hat{Q}_h(s, a)$ 
10:  Set  $\pi_h(s) \leftarrow \arg \max_{a \in \mathcal{A}} \hat{Q}_h(s, a)$ 
11: end for
12: Return  $\pi_1, \dots, \pi_H$ 

```

---

## 5 Polynomial Realizability

In this section, we study the sample complexity to learn deterministic MDPs under polynomial realizability. We identify sufficient and necessary conditions for efficiently learning the MDPs for two different settings — the generative model setting and the online RL setting. Specifically, we show that if the image of the feature map  $\phi_h(s_h, a_h)$  satisfies some positive measure conditions, then by random exploring we can identify the optimal policy with samples that is linear in the algebraic dimension of the underlying polynomial class. We also provide a lower bound example showing the separation between the two settings.

Next, we introduce the notion of **Admissible Polynomial Families**, which are the families of structured polynomial that enables efficient learning.

**Definition 5.1** (Admissible Polynomial Families). For  $x \in \mathbb{R}^d$ , denote  $\tilde{x} = [1, x^\top]^\top$ . Let  $\mathcal{X} := \{\tilde{x}^{\otimes p} : x \in \mathbb{R}^d\}$ . For any algebraic variety  $\mathcal{V}$ , we define  $\mathcal{F}_\mathcal{V} := \{f_\Theta(x) = \langle \Theta, \tilde{x}^{\otimes p} \rangle : \Theta \in \mathcal{V}\}$  as the polynomial family parameterized by  $\Theta \in \mathcal{V}$ . We say  $\mathcal{F}_\mathcal{V}$  is admissible<sup>3</sup> w.r.t.  $\mathcal{X}$ , if for any  $\Theta \in \mathcal{V}$ ,  $\dim(\mathcal{X} \cap \{X \in \mathcal{X} : \langle X, \Theta \rangle = 0\}) < \dim(\mathcal{X}) = d$ . We define the dimension  $D$  of the family to be the dimension of  $\mathcal{V}$ .

Next theorem shows that to learn an admissible polynomial family, the sample complexity only scales with the algebraic dimension of the polynomial family.

**Theorem 5.2** (Anonymous). *Consider the polynomial family  $\mathcal{F}_\mathcal{V}$  of dimension  $D$ . For  $n \geq 2D$ , there exists a Lebesgue-measure zero set  $N \in \mathbb{R}^d \times \dots \times \mathbb{R}^d$ , such that if  $(x_1, \dots, x_n) \notin N$ , for any  $y_i$ , there is a unique  $f$  (or no such  $f$ ) to the system of equations  $y_i = f(x_i)$  for  $f \in \mathcal{F}_\mathcal{V}$ .*

We give two important examples of admissible polynomial families with low dimension.

**Example 5.3.** (Low-rank Polynomial of rank  $k$ ) The function  $f \in \mathcal{F}_\mathcal{V}$  is a polynomial with  $k$  terms, that is

$$F(x) = \sum_{i=1}^k \lambda_i \langle v_i, x \rangle^{p_i},$$

where  $p = \max\{p_i\}$ . The dimension of this family is upper bounded by  $D \leq dk$ . Neural network with monomial/polynomial activation functions are low-rank polynomials.

**Example 5.4.** The function  $f \in \mathcal{F}_\mathcal{V}$  is of the form  $f(x) = q(Ux)$ , where  $U \in \mathbb{R}^{k \times d}$  and  $q$  is a degree  $p$  polynomial. The polynomial  $q$  and matrix  $U$  are unknown. The dimension of this family is upper bounded by  $D \leq d(k+1)^p$ .

Next we introduce the notion of positive measure.

---

<sup>3</sup>Admissible means the dimension of  $\mathcal{X}$  decreases by one when there is an additional linear constraint  $\langle \Theta, X \rangle = 0$

**Definition 5.5.** We say a measurable set  $E \in \mathbb{R}^d$  is of positive measure, if  $\mu(E) > 0$ , where  $\mu$  is the standard Lebesgue measure on  $\mathbb{R}^d$ .

If a measurable set  $E$  satisfies  $\mu(E) > 0$ , then there exists a procedure to draw samples from  $E$ , such that for any  $N \subset \mathbb{R}^d$  of Lebesgue-measure zero, the probability that the sample falls in  $N$  is zero. In fact, the sampling probability can be given by  $\mathbb{P}_{x \in \mathcal{N}(0, I_d)}(\cdot | x \in E)$ . The intuition behind is definition is that for all admissible polynomial families, the set of  $(x_1, \dots, x_n)$  that has "redundant information" about learning the parameter  $\Theta$  is of Lebesgue-measure zero. Therefore, a positive measure set allows you to query randomly and avoids getting coherent measurements.

Next two theorems identify the sufficient conditions for efficiently learning deterministic MDPs under polynomial realizability. Specifically, under online RL setting, we require the strong assumption that the set  $\{\phi_h(s, a) | a \in \mathcal{A}\}$  is of positive measure for all  $h \in [H]$  and all  $s \in \mathcal{S}$ , while under generative model setting, we only require the union set  $\bigcup_{s \in \mathcal{S}} \{\phi_h(s, a) | a \in \mathcal{A}\}$  to be of positive measure for all  $h \in [H]$ . The algorithms for solving the both cases are summarized in Algorithms 4 and 5.

**Assumption 5.6** (Polynomial Realizability). For all  $h \in [H]$ ,  $Q_h^*(s_h, a_h)$ , viewed as the function of  $\phi_h(s_h, a_h)$ , lies in some admissible polynomial family  $\mathcal{F}_{V_h}$  with dimension bounded by  $D$ .

**Theorem 5.7.** For the generative model setting, assume that the set  $\{\phi_h(s, a) | s \in \mathcal{S}, a \in \mathcal{A}\}$  is of positive measure at any level  $h$ . Under the polynomial realizability, Algorithm 4 almost surely learns the optimal policy  $\pi^*$  with at most  $N = 2DH$  samples.

**Theorem 5.8.** For the online RL setting, assume that  $\{\phi_h(s, a) | a \in \mathcal{A}\}$  is of positive measure for every state  $s$  at every level  $h$ . Under polynomial realizability, within  $T = 2DH$  episodes, Algorithm 5 learns the optimal policy  $\pi^*$  almost surely.

---

**Algorithm 4** Dynamic programming under generative model settings

---

```

1: for  $h = H, \dots, 1$  do
2:   1. Sample  $2D$  points  $\{\phi_h(s_h^{(i)}, a_h^{(i)})\}_{i=1}^{2D}$  according to  $\mathbb{P}_{x \in \mathcal{N}(0, I_d)}(\cdot | x \in E_h)$  where  $E_h = \{\phi_h(s, a) | s \in \mathcal{S}, a \in \mathcal{A}\}$ .
3:   2. Query the generative model with state-action pair  $(s_h^{(i)}, a_h^{(i)})$  at level  $h$  for  $i = 1, \dots, 2D$ , and observe the next state  $\tilde{s}_h^{(i)}$  and reward  $r_h^{(i)}$ .
4:   3. Solve for  $Q_h^*$  with the  $2D$  equations  $Q_h^*(s_h^{(i)}, a_h^{(i)}) = r_h^{(i)} + V_{h+1}^*(\tilde{s}_h^{(i)})$ .
5:   4. Set  $\pi_h^*(s) = \arg \max_a Q_h^*(s, a)$  and  $V_h^*(s) = \max_a Q_h^*(s, a)$ .
6: end for
7: Output  $\pi^*$ 

```

---



---

**Algorithm 5** Dynamic programming under online RL settings

---

```

1: for  $h = H, \dots, 1$  do
2:   1. Fix any action sequence  $a_1, \dots, a_{h-1}$ .
3:   2. Play  $a_1, \dots, a_{h-1}$  for the first  $h-1$  levels and reaches a state  $s_h$ . Sample  $2D$  points  $\{\phi_h(s_h, a_h^{(i)})\}_{i=1}^{2D}$  according to  $\mathbb{P}_{x \in \mathcal{N}(0, I_d)}(\cdot | x \in E_h)$  where  $E_h = \{\phi_h(s_h, a) | a \in \mathcal{A}\}$ .
4:   3. play  $a_h^{(i)}$  at  $s_h$  for  $i = 1, \dots, 2D$ , and observe the next state  $\tilde{s}_h^{(i)}$  and reward  $r_h^{(i)}$ .
5:   4. Solve for  $Q_h^*$  with the  $2D$  equations  $Q_h^*(s_h^{(i)}, a_h^{(i)}) = r_h^{(i)} + V_{h+1}^*(\tilde{s}_h^{(i)})$ .
6:   5. Set  $\pi_h^*(s) = \arg \max_a Q_h^*(s, a)$  and  $V_h^*(s) = \max_a Q_h^*(s, a)$ .
7: end for
8: Output  $\pi^*$ 

```

---

We remark that our Theorem 5.8 for learning MDPs under the online RL setting relies on a very strong assumption that allows the learner to explore randomly for any state. However, in some sense this assumption is necessary, as is suggested by our lower bound example in the next subsection.



## 5.1 Necessity of Generic Feature Maps in Online RL

In this section, we consider lower bounds for learning deterministic MDPs with polynomial realizable  $Q^*$  under online RL setting. Our goal is to show that in the online setting the generic assumption on the feature maps  $\phi_h(s, \cdot)$  is necessary. On the contrary, under the generative model setting one can efficiently learn the MDPs without such a strong assumption, since at every level  $h$  we can set the state arbitrarily.

**MDP construction** We briefly introduce the intuition of our construction. Consider a family of MDPs with only two states  $\mathcal{S} = \{S_{\text{good}}, S_{\text{bad}}\}$ . we set the feature map  $\phi_h$  such that, for the good state  $S_{\text{good}}$ , it allows the learner to explore randomly, i.e.,  $\{\phi_h(S_{\text{good}}, a) \mid a \in \mathcal{A}\}$  is of positive measure. However, for the bad state  $S_{\text{bad}}$ , all actions are mapped to some restricted set, which forbids random exploration, i.e.,  $\{\phi_h(S_{\text{bad}}, a) \mid a \in \mathcal{A}\}$  is measure zero. This is illustrated in Figure 1. Specifically, at least  $\Omega(d^p)$  actions are needed to identify the ground-truth polynomial of  $Q_h^*$  for  $S_{\text{bad}}$ , while  $O(d)$  actions suffice for  $S_{\text{good}}$ . The transition  $\mathbb{P}_h$  is constructed as  $\mathbb{P}_h(s_{\text{bad}} \mid s, a) = 1$  for all  $s \in \mathcal{S}, a \in \mathcal{A}$ , which means it is impossible for the online scenarios to reach the good state for  $h > 1$ .

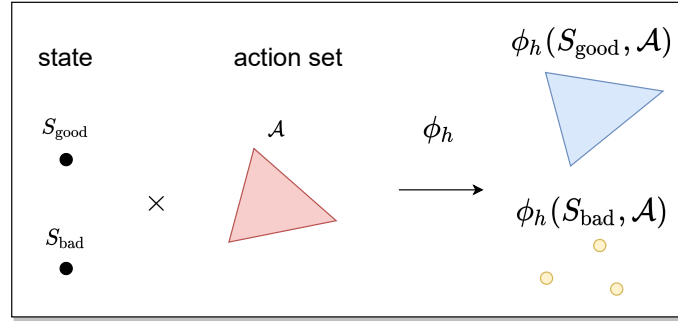

Figure 1: An illustration of the hard case for deterministic MDPs with polynomial realizable  $Q^*$ . The image of the feature map  $\phi_h$  at  $S_{\text{good}}$  is of positive measure, while the image of  $\phi_h$  at  $S_{\text{bad}}$  is not. This makes it difficult to learn under the online RL setting.

**Theorem 5.9.** *There exists a family of MDPs satisfying Assumption 5.6, such that the set  $\{\phi_h(s, a) \mid s \in \mathcal{S}, a \in \mathcal{A}\}$  is of positive measure at any level  $h$ , but for all  $h$  there is some  $s_{\text{bad}} \in \mathcal{S}$  such that  $\{\phi_h(s_{\text{bad}}, a) \mid a \in \mathcal{A}\}$  is measure zero. Under the online RL setting, any algorithm needs to play at least  $\Omega(d^p)$  episodes to identify the optimal policy. On the contrary, under the generative model setting, only  $O(d)H$  samples are needed.*

## 6 Conclusions

In this paper, we consider neural network and polynomial function approximation in the simulator setting. To our knowledge, this is the first paper that shows sample-efficient reinforcement learning is possible with neural net function approximation. Our results substantially improve upon what can be achieved with existing results that primarily rely on embedding neural networks into linear function classes.

Our results for polynomial activation require deterministic transitions, since we cannot handle how noise propagates in solving polynomial equations. We leave to future work an in-depth studying of the stability of roots of polynomial systems with noise, which is a fundamental mathematical problem. We believe that noisy tensor decomposition approaches combined with zeroth order optimization may allow for stochastic transitions.

In the online RL setting, we are only able to show efficient learning under a very strong yet necessary assumption on the feature mapping. We leave to future work identifying more realistic and natural conditions which permit efficient learning in the online RL setting.

## References

- Yasin Abbasi-Yadkori, Dávid Pál, and Csaba Szepesvári. Improved algorithms for linear stochastic bandits. In *Advances in Neural Information Processing Systems*, pages 2312–2320, 2011.
- Yasin Abbasi-Yadkori, Nevena Lazic, Csaba Szepesvari, and Gellert Weisz. Exploration-enhanced POLITEX. *arXiv preprint arXiv:1908.10479*, 2019.
- Zeyuan Allen-Zhu, Yuanzhi Li, and Zhao Song. A convergence theory for deep learning via over-parameterization. In *International Conference on Machine Learning (ICML)*, pages 242–252, 2019.
- Anonymous. Anonymous submission by same authors.
- Mohammad Gheshlaghi Azar, Ian Osband, and Rémi Munos. Minimax regret bounds for reinforcement learning. In *Proceedings of the 34th International Conference on Machine Learning*, pages 263–272, 2017.
- Christopher Berner, Greg Brockman, Brooke Chan, Vicki Cheung, Przemyslaw Debiak, Christy Dennison, David Farhi, Quirin Fischer, Shariq Hashme, and Chris Hesse. Dota 2 with large scale deep reinforcement learning. *arXiv preprint arXiv:1912.06680*, 2019.
- Christoph Dann, Nan Jiang, Akshay Krishnamurthy, Alekh Agarwal, John Langford, and Robert E. Schapire. On oracle-efficient PAC-RL with rich observations. In *Advances in Neural Information Processing Systems*, 2018.
- Kefan Dong, Jian Peng, Yining Wang, and Yuan Zhou.  $\sqrt{n}$ -regret for learning in Markov decision processes with function approximation and low Bellman rank. In *Conference on Learning Theory*, pages 1554–1557. PMLR, 2020.
- Kefan Dong, Jiaqi Yang, and Tengyu Ma. Provable model-based nonlinear bandit and reinforcement learning: Shelf optimism, embrace virtual curvature. *arXiv preprint arXiv:2102.04168*, 2021.
- Simon Du, Jason Lee, Haochuan Li, Liwei Wang, and Xiyu Zhai. Gradient descent finds global minima of deep neural networks. In *International Conference on Machine Learning (ICML)*, pages 1675–1685. PMLR, 2019a.
- Simon S Du, Akshay Krishnamurthy, Nan Jiang, Alekh Agarwal, Miroslav Dudik, and John Langford. Provably efficient RL with rich observations via latent state decoding. In *International Conference on Machine Learning*, pages 1665–1674, 2019b.
- Simon S Du, Sham M Kakade, Ruosong Wang, and Lin F Yang. Is a good representation sufficient for sample efficient reinforcement learning? In *International Conference on Learning Representations*, 2020a.
- Simon S. Du, Sham M. Kakade, Ruosong Wang, and Lin F. Yang. Is a good representation sufficient for sample efficient reinforcement learning? In *International Conference on Learning Representations*, 2020b.
- Simon S Du, Jason D Lee, Gaurav Mahajan, and Ruosong Wang. Agnostic Q-learning with function approximation in deterministic systems: Tight bounds on approximation error and sample complexity. *Advances in Neural Information Processing Systems*, 2020c.
- Simon S. Du, Sham M. Kakade, Jason D. Lee, Shachar Lovett, Gaurav Mahajan, Wen Sun, and Ruosong Wang. Bilinear classes: A structural framework for provable generalization in rl. *arXiv preprint arXiv:2103.10897*, 2021.
- Rong Ge, Jason D. Lee, and Tengyu Ma. Learning one-hidden-layer neural networks with landscape design. *arXiv preprint arXiv:1711.00501*, 2017.

Behrooz Ghorbani, Song Mei, Theodor Misiakiewicz, and Andrea Montanari. Linearized two-layers neural networks in high dimension. *The Annals of Statistics*, 49(2):1029–1054, 2021.

Ian Goodfellow, Yoshua Bengio, and Aaron Courville. *Deep learning*. MIT press, 2016.

Peter Henderson, Riashat Islam, Philip Bachman, Joelle Pineau, Doina Precup, and David Meger. Deep reinforcement learning that matters. In *Proceedings of the AAAI Conference on Artificial Intelligence*, volume 32, 2018.

Arthur Jacot, Franck Gabriel, and Clément Hongler. Neural tangent kernel: Convergence and generalization in neural networks. In *Advances in neural information processing systems (NeurIPS)*, pages 8571–8580, 2018.

Thomas Jaksch, Ronald Ortner, and Peter Auer. Near-optimal regret bounds for reinforcement learning. *Journal of Machine Learning Research*, 11(Apr):1563–1600, 2010.

Majid Janzamin, Hanie Sedghi, and Anankumar Anima. Beating the perils of nonconvexity: Guaranteed training of neural networks using tensor methods. arXiv preprint arXiv:1506.08473, 2015.

Nan Jiang, Akshay Krishnamurthy, Alekh Agarwal, John Langford, and Robert E Schapire. Contextual decision processes with low Bellman rank are PAC-learnable. In *Proceedings of the 34th International Conference on Machine Learning*, pages 1704–1713, 2017.

Chi Jin, Zeyuan Allen-Zhu, Sebastien Bubeck, and Michael I Jordan. Is Q-learning provably efficient? In *Advances in Neural Information Processing Systems*, pages 4863–4873, 2018.

Chi Jin, Zhuoran Yang, Zhaoran Wang, and Michael I Jordan. Provably efficient reinforcement learning with linear function approximation. In *Conference on Learning Theory*, pages 2137–2143. PMLR, 2020a.

Chi Jin, Zhuoran Yang, Zhaoran Wang, and Michael I Jordan. Provably efficient reinforcement learning with linear function approximation. In *Conference on Learning Theory*, pages 2137–2143, 2020b.

Chi Jin, Qinghua Liu, and Sobhan Miryoosefi. Bellman eluder dimension: New rich classes of rl problems, and sample-efficient algorithms. arXiv preprint arXiv:2102.00875, 2021.

Sham Machandranath Kakade. *On the sample complexity of reinforcement learning*. PhD thesis, University of College London, 2003.

Volodymyr Kuleshov, Arun Chaganty, and Percy Liang. Tensor factorization via matrix factorization. In *Proceedings of the Eighteenth International Conference on Artificial Intelligence and Statistics (AISTATS)*, page 507–516, 2015.

Yann LeCun, Yoshua Bengio, and Geoffrey Hinton. Deep learning. *Nature*, 521(7553):436–444, 2015.

Timothy P Lillicrap, Jonathan J Hunt, Alexander Pritzel, Nicolas Heess, Tom Erez, Yuval Tassa, David Silver, and Daan Wierstra. Continuous control with deep reinforcement learning. *arXiv preprint arXiv:1509.02971*, 2015.

Boyi Liu, Qi Cai, Zhuoran Yang, and Zhaoran Wang. Neural proximal/trust region policy optimization attains globally optimal policy. arXiv preprint arXiv:1906.10306, 2019.

Volodymyr Mnih, Koray Kavukcuoglu, David Silver, Alex Graves, Ioannis Antonoglou, Daan Wierstra, and Martin Riedmiller. Playing atari with deep reinforcement learning. arXiv preprint arXiv:1312.5602, 2013a.

Volodymyr Mnih, Koray Kavukcuoglu, David Silver, Alex Graves, Ioannis Antonoglou, Daan Wierstra, and Martin Riedmiller. Playing Atari with deep reinforcement learning. *arXiv preprint arXiv:1312.5602*, 2013b.

386 Matej Moravčík, Martin Schmid, Neil Burch, Viliam Lisý, Dustin Morrill, Nolan Bard, Trevor  
387 Davis, Kevin Waugh, Michael Johanson, and Michael Bowling. Deepstack: Expert-level artificial  
388 intelligence in heads-up no-limit poker. *Science*, 356(6337):508–513, 2017.

389 Ian Osband, Daniel Russo, and Benjamin Van Roy. (more) efficient reinforcement learning via  
390 posterior sampling. In *Advances in Neural Information Processing Systems*, pages 3003–3011,  
391 2013.

392 Alexander Rakhlin, Karthik Sridharan, and Ambuj Tewari. Online learning via sequential complexi-  
393 ties. *Journal of Machine Learning Research*, 16(6):155–186, 2015a.

394 Alexander Rakhlin, Karthik Sridharan, and Ambuj Tewari. Sequential complexities and uniform  
395 martingale laws of large numbers. *Probability Theory and Related Fields*, 161(1-2):111–153,  
396 2015b.

397 Dan Russo and Benjamin Van Roy. Eluder dimension and the sample complexity of optimistic  
398 exploration. In *Advances in Neural Information Processing Systems*, pages 2256–2264, 2013a.

399 Daniel Russo. Worst-case regret bounds for exploration via randomized value functions. In *Advances*  
400 *in Neural Information Processing Systems*, pages 14433–14443, 2019.

401 Daniel Russo and Benjamin Van Roy. Eluder dimension and the sample complexity of optimistic  
402 exploration. In *Advances in Neural Information Processing Systems*, 2013b.

403 Igor R Shafarevich. *Basic Algebraic Geometry 1: Varieties in Projective Space*. Springer Science &  
404 Business Media, 2013.

405 Shai Shalev-Shwartz, Shaked Shammah, and Amnon Shashua. Safe, multi-agent, reinforcement  
406 learning for autonomous driving. *arXiv preprint arXiv:1610.03295*, 2016.

407 Aaron Sidford, Mengdi Wang, Xian Wu, Lin F Yang, and Yinyu Ye. Near-optimal time and sample  
408 complexities for solving discounted markov decision process with a generative model. *arXiv*  
409 *preprint arXiv:1806.01492*, 2018.

410 David Silver, Aja Huang, Chris J. Maddison, Arthur Guez, Laurent Sifre, George Van Den Driessche,  
411 Julian Schrittwieser, Ioannis Antonoglou, Veda Panneershelvam, and Marc Lanctot. Mastering the  
412 game of Go with deep neural networks and tree search. *Nature*, 529(7587):484, 2016.

413 Alexander L Strehl, Lihong Li, Eric Wiewiora, John Langford, and Michael L Littman. PAC model-  
414 free reinforcement learning. In *Proceedings of the 23rd international conference on Machine*  
415 *learning*, pages 881–888. ACM, 2006.

416 Wen Sun, Nan Jiang, Akshay Krishnamurthy, Alekh Agarwal, and John Langford. Model-based  
417 RL in contextual decision processes: PAC bounds and exponential improvements over model-free  
418 approaches. In *Conference on Learning Theory*, pages 2898–2933, 2019.

419 Richard S Sutton and Andrew G. Barto. *Reinforcement learning: An introduction*. MIT press, 2018.

420 Lingxiao Wang, Qi Cai, Zhuoran Yang, and Zhaoran Wang. Neural policy gradient methods: Global  
421 optimality and rates of convergence. *arXiv preprint arXiv:1909.01150*, 2020a.

422 Ruosong Wang, Ruslan Salakhutdinov, and Lin F Yang. Provably efficient reinforcement learning  
423 with general value function approximation. *arXiv preprint arXiv:2005.10804*, 2020b.

424 Yining Wang, Ruosong Wang, Simon S. Du, and Akshay Krishnamurthy. Optimism in reinforcement  
425 learning with generalized linear function approximation. In *International Conference on Learning*  
426 *Representations*, 2021a.

427 Yuanhao Wang, Ruosong Wang, and Sham M. Kakade. An exponential lower bound for linearly-  
428 realizable mdps with constant suboptimality gap. *arXiv preprint arXiv:2103.12690*, 2021b.

- 429 Gellert Weisz, Philip Amortila, and Csaba Szepesvári. Exponential lower bounds for planning in  
430 mdps with linearly-realizable optimal action-value functions. *arXiv preprint arXiv:2010.01374*,  
431 2020.
- 432 Zheng Wen and Benjamin Van Roy. Efficient reinforcement learning in deterministic systems with  
433 value function generalization. *Math. Oper. Res.*, 42(3):762–782, 2017. ISSN 0364-765X.
- 434 Lin F Yang and Mengdi Wang. Reinforcement leaning in feature space: Matrix bandit, kernels, and  
435 regret bound. *International Conference on Machine Learning*, 2020.
- 436 Andrea Zanette and Emma Brunskill. Tighter problem-dependent regret bounds in reinforcement  
437 learning without domain knowledge using value function bounds. In *International Conference on*  
438 *Machine Learning*, pages 7304–7312, 2019.
- 439 Andrea Zanette, Alessandro Lazaric, Mykel Kochenderfer, and Emma Brunskill. In *International*  
440 *Conference on Machine Learning*, 2020.
- 441 Kai Zhong, Zhao Song, Prateek Jain, Peter L. Bartlett, and Inderjit S. Dhillon. Recovery guarantees  
442 for one-hidden-layer neural networks. *Proceedings of the Thirty-fourth International Conference*  
443 *on Machine Learning (ICML)*, 70, 2017.

## 444 Checklist

- 445 1. For all authors...
- 446 (a) Do the main claims made in the abstract and introduction accurately reflect the paper’s  
447 contributions and scope? [Yes] Our abstract and introduction accurately reflect our  
448 main contribution.
- 449 (b) Did you describe the limitations of your work? [Yes] In the Preliminary section we  
450 clearly state the settings we considered and when our results apply.
- 451 (c) Did you discuss any potential negative societal impacts of your work? [No] Our work  
452 is theoretical and generally will not have negative social impacts.
- 453 (d) Have you read the ethics review guidelines and ensured that your paper conforms to  
454 them? [Yes]
- 455 2. If you are including theoretical results...
- 456 (a) Did you state the full set of assumptions of all theoretical results? [Yes] The assump-  
457 tions are clearly included in every theorem or lemma.
- 458 (b) Did you include complete proofs of all theoretical results? [Yes] All the proofs can be  
459 found in the appendix
- 460 3. If you ran experiments...
- 461 (a) Did you include the code, data, and instructions needed to reproduce the main experi-  
462 mental results (either in the supplemental material or as a URL)? [N/A]
- 463 (b) Did you specify all the training details (e.g., data splits, hyperparameters, how they  
464 were chosen)? [N/A]
- 465 (c) Did you report error bars (e.g., with respect to the random seed after running experi-  
466 ments multiple times)? [N/A]
- 467 (d) Did you include the total amount of compute and the type of resources used (e.g., type  
468 of GPUs, internal cluster, or cloud provider)? [N/A]
- 469 4. If you are using existing assets (e.g., code, data, models) or curating/releasing new assets...
- 470 (a) If your work uses existing assets, did you cite the creators? [N/A]
- 471 (b) Did you mention the license of the assets? [N/A]
- 472 (c) Did you include any new assets either in the supplemental material or as a URL? [N/A]
- 473

- 474 (d) Did you discuss whether and how consent was obtained from people whose data you're  
475 using/curating? [N/A]
- 476 (e) Did you discuss whether the data you are using/curating contains personally identifiable  
477 information or offensive content? [N/A]
- 478 5. If you used crowdsourcing or conducted research with human subjects...
- 479 (a) Did you include the full text of instructions given to participants and screenshots, if  
480 applicable? [N/A]
- 481 (b) Did you describe any potential participant risks, with links to Institutional Review  
482 Board (IRB) approvals, if applicable? [N/A]
- 483 (c) Did you include the estimated hourly wage paid to participants and the total amount  
484 spent on participant compensation? [N/A]

## 485 A Proof of Section 4

### 486 A.1 Proof of Theorem 4.4

487 *Proof.* Use  $\pi_1^*, \dots, \pi_H^*$  to denote the global optimal policy. We prove that Algorithm 1 learns  $\pi_h^*$   
488 from  $h = H$  to  $h = 1$ .

489 At level  $H$ , the query obtains exact  $Q_H^*(s, a)$ . Therefore by Theorem A.12,  $\hat{Q}_H = Q_H^*$  and thus  
490 the optimal planning finds  $\pi_H = \pi_H^*$ . Suppose we have learned  $\pi_{h+1}^*, \dots, \pi_H^*$  at level  $h$ . Due to  
491 deterministic transition, the query obtains exact  $Q_h^*(s, a)$ . Therefore by Theorem A.12,  $\hat{Q}_h = Q_h^*$  and  
492 thus the optimal planning finds  $\pi_h = \pi_h^*$ . Recursively applying this process to  $h = 1$ , we complete  
493 the proof.  $\square$

### 494 A.2 Proof of Theorem 4.5

495 *Proof.* Use  $\pi_1^*, \dots, \pi_H^*$  to denote the global optimal policy. We prove for all  $s \in \mathcal{S}$ ,

$$V_h^{\pi_h^*, \pi_{h+1}^*, \dots, \pi_H^*}(s) - V_h^{\pi_h, \pi_{h+1}, \dots, \pi_H}(s) \leq \frac{(H - h + 1)\epsilon}{H}.$$

496 At level  $H$ , let  $e_H(s_H^i, a_H^i) = r_H(s_H^i, a_H^i) - Q_H^*(s_H^i, a_H^i)$ , then  $e_H(s_H^i, a_H^i) = 0$ . From Theo-  
497 rem A.10, we have  $\hat{Q}_H(s, a) := v_H^\top \sigma(W_H \phi(s, a))$  satisfies  $|\hat{Q}_H(s, a) - Q_H^*(s, a)| \leq \frac{\epsilon}{2H}$  for all  
498  $s \in \mathcal{S}, a \in \mathcal{A}$ . Therefore for all  $s \in \mathcal{S}$ ,

$$\begin{aligned} V_H^*(s) - V_H^{\pi_H}(s) &= \mathbb{E}_{a \sim \pi_H^*}[Q_H^*(s, a)] - \mathbb{E}_{a \sim \pi_H^*}[\hat{Q}_H(s, a)] \\ &\quad + \mathbb{E}_{a \sim \pi_H^*}[\hat{Q}_H(s, a)] - \mathbb{E}_{a \sim \pi_H}[\hat{Q}_H(s, a)] \\ &\quad + \mathbb{E}_{a \sim \pi_H}[\hat{Q}_H(s, a)] - \mathbb{E}_{a \sim \pi_H}[Q_H^*(s, a)] \\ &\leq \frac{\epsilon}{H} \end{aligned}$$

499 where in the second step we used  $\mathbb{E}_{a \sim \pi_H^*}[\hat{Q}_H(s, a)] \leq \mathbb{E}_{a \sim \pi_H}[\hat{Q}_H(s, a)]$  by optimality of  $\pi_H$  and  
500  $|\hat{Q}_H(s, a) - Q_H^*(s, a)| \leq \frac{\epsilon}{2H}$ .

Suppose we have learned policies  $\pi_{h+1}, \dots, \pi_H$ , we use  $\tilde{\pi}_h$  to denote the optimal policy of  $Q_h^{\pi_{h+1}, \dots, \pi_H}(s, a)$ . Let

$$e_h(s_h^i, a_h^i) = \hat{Q}_h^{\pi_{h+1}, \dots, \pi_H}(s_h^i, a_h^i) - Q_h^{\pi_{h+1}, \dots, \pi_H}(s_h^i, a_h^i)$$

501 then  $e_h(s_h^i, a_h^i)$  is zero mean  $H^2$  sub-Gaussian (notice that  $\hat{Q}_h^{\pi_{h+1}, \dots, \pi_H}(s_h^i, a_h^i)$  is unbiased estimate  
502 of  $Q_h^{\pi_{h+1}, \dots, \pi_H}(s_h^i, a_h^i)$ , and  $\hat{Q}_h^{\pi_{h+1}, \dots, \pi_H}(s_h^i, a_h^i) \leq H$ ). From Theorem A.10, we have  $\hat{Q}_h(s, a) :=$   
503  $v_h^\top \sigma(W_h \phi(s, a))$  satisfies  $|\hat{Q}_h(s, a) - Q_h^{\pi_{h+1}, \dots, \pi_H}(s, a)| \leq \frac{\epsilon}{2H}$  for all  $s \in \mathcal{S}, a \in \mathcal{A}$ . Therefore for  
504 all  $s \in \mathcal{S}$ ,

$$\begin{aligned} &V_h^{\tilde{\pi}_h, \pi_{h+1}, \dots, \pi_H}(s) - V_h^{\pi_h, \pi_{h+1}, \dots, \pi_H}(s) \\ &= \mathbb{E}_{a \sim \tilde{\pi}_h}[Q_h^{\pi_{h+1}, \dots, \pi_H}(s, a)] - \mathbb{E}_{a \sim \tilde{\pi}_h}[\hat{Q}_h(s, a)] \\ &\quad + \mathbb{E}_{a \sim \tilde{\pi}_h}[\hat{Q}_h(s, a)] - \mathbb{E}_{a \sim \pi_h}[\hat{Q}_h(s, a)] \\ &\quad + \mathbb{E}_{a \sim \pi_h}[\hat{Q}_h(s, a)] - \mathbb{E}_{a \sim \pi_h}[Q_h^{\pi_{h+1}, \dots, \pi_H}(s, a)] \\ &\leq \frac{\epsilon}{H} \end{aligned}$$

505 where in the second step we used  $\mathbb{E}_{a \sim \tilde{\pi}_h}[\hat{Q}_h(s, a)] \leq \mathbb{E}_{a \sim \pi_h}[\hat{Q}_h(s, a)]$  by optimality of  $\pi_h$  and  
506  $|\hat{Q}_h(s, a) - Q_h^{\pi_{h+1}, \dots, \pi_H}(s, a)| \leq \frac{\epsilon}{2H}$ .

Therefore for all  $s \in \mathcal{S}$ ,

$$\begin{aligned}
V_h^{\pi_h^*, \pi_{h+1}^*, \dots, \pi_H^*}(s) - V_h^{\pi_h, \pi_{h+1}, \dots, \pi_H}(s) &= V_h^{\pi_h^*, \pi_{h+1}^*, \dots, \pi_H^*}(s) - V_h^{\pi_h^*, \pi_{h+1}, \dots, \pi_H}(s) \\
&\quad + V_h^{\pi_h^*, \pi_{h+1}, \dots, \pi_H}(s) - V_h^{\tilde{\pi}_h, \pi_{h+1}, \dots, \pi_H}(s) \\
&\quad + V_h^{\tilde{\pi}_h, \pi_{h+1}, \dots, \pi_H}(s) - V_h^{\pi_h, \pi_{h+1}, \dots, \pi_H}(s) \\
&\leq V_h^{\pi_h^*, \pi_{h+1}^*, \dots, \pi_H^*}(s) - V_h^{\pi_h^*, \pi_{h+1}, \dots, \pi_H}(s) + \frac{\epsilon}{H} \\
&\leq \dots \\
&\leq \frac{(H-h+1)\epsilon}{H}.
\end{aligned}$$

where in the second step we use  $V_h^{\pi_h^*, \pi_{h+1}, \dots, \pi_H}(s) \leq V_h^{\tilde{\pi}_h, \pi_{h+1}, \dots, \pi_H}(s)$  from optimality of  $\tilde{\pi}_h$ .  $\square$

### A.3 Proof of Theorem 4.6

*Proof.* Use  $\pi_1^*, \dots, \pi_H^*$  to denote the global optimal policy. We prove

$$|\hat{Q}_h(s, a) - Q_h^*(s, a)| \leq \frac{(H-h+1)\epsilon}{H} \quad (1)$$

for all  $s \in \mathcal{S}, a \in \mathcal{A}$ .

At level  $H$ , let

$$e_H(s_H^i, a_H^i) = r_H(s_H^i, a_H^i) - Q_H^*(s_H^i, a_H^i)$$

then  $e_H(s_H^i, a_H^i) = 0$ . From Theorem A.10, we have  $\hat{Q}_H(s, a) := v_H^\top \sigma(W_H \phi(s, a))$  satisfies

$|\hat{Q}_H(s, a) - Q_H^*(s, a)| \leq \frac{\epsilon}{H}$  for all  $s \in \mathcal{S}, a \in \mathcal{A}$ .

Suppose we have learned  $\hat{Q}_{h+1}(s, a)$  with  $|\hat{Q}_{h+1}(s, a) - Q_{h+1}^*(s, a)| \leq \frac{(H-h)\epsilon}{H}$ . At level  $h$ , let

$$e_h(s_h^i, a_h^i) = r_h(s_h^i, a_h^i) + \hat{V}_{h+1}(s_{h+1}^i) - \mathcal{T}_h(\hat{Q}_{h+1})(s_h^i, a_h^i)$$

then  $e_h(s_h^i, a_h^i)$  is zero mean  $H^2$  sub-Gaussian (notice that  $r_h(s_h^i, a_h^i) + \hat{V}_{h+1}(s_{h+1}^i)$  is unbiased

estimate of  $\mathcal{T}_h(\hat{Q}_{h+1})(s_h^i, a_h^i)$ , and  $r_h(s_h^i, a_h^i) + \hat{V}_{h+1}(s_{h+1}^i) \leq H$ ). From Theorem A.10, we have

$\hat{Q}_H(s, a) := v_H^\top \sigma(W_H \phi(s, a))$  satisfies  $|\hat{Q}_H(s, a) - \mathcal{T}_h(\hat{Q}_{h+1})(s_h^i, a_h^i)| \leq \frac{\epsilon}{H}$  for all  $s \in \mathcal{S}, a \in \mathcal{A}$ .

Therefore

$$\begin{aligned}
|\hat{Q}_h(s, a) - Q_h^*(s, a)| &\leq |\hat{Q}_h(s, a) - \mathcal{T}_h(\hat{Q}_{h+1})(s, a)| + |\mathcal{T}_h(\hat{Q}_{h+1})(s, a) - Q_h^*(s, a)| \\
&\leq \frac{\epsilon}{H} + \max_{s \in \mathcal{S}, a \in \mathcal{A}} |\hat{Q}_{h+1}(s, a) - Q_{h+1}^*(s, a)| \\
&\leq \frac{(H-h+1)\epsilon}{H}
\end{aligned}$$

holds for all  $s \in \mathcal{S}, a \in \mathcal{A}$ .

It thus follows that for all  $s_1 \in \mathcal{S}$ ,

$$\begin{aligned}
V_h^{\pi_1^*, \dots, \pi_H^*}(s_1) - V_h^{\pi_1, \dots, \pi_H}(s_1) &= \mathbb{E}_{a \sim \pi_1^*}[Q_1^*(s_1, a)] - \mathbb{E}_{a \sim \pi_1}[Q_1^{\pi_2, \dots, \pi_H}(s_1, a)] \\
&\leq \mathbb{E}_{a \sim \pi_1^*}[\hat{Q}_1(s_1, a)] - \mathbb{E}_{a \sim \pi_1}[Q_1^{\pi_2, \dots, \pi_H}(s_1, a)] + \epsilon \\
&\leq \mathbb{E}_{a \sim \pi_1}[\hat{Q}_1(s_1, a) - Q_1^{\pi_2, \dots, \pi_H}(s_1, a)] + \epsilon \\
&\leq \mathbb{E}_{a \sim \pi_1}[Q_1^*(s_1, a) - Q_1^{\pi_2, \dots, \pi_H}(s_1, a)] + 2\epsilon \\
&\leq \mathbb{E}_{a \sim \pi_1} \mathbb{E}_{s_2 \sim \mathbb{P}(\cdot | s_1, a)}[V_2^{\pi_2^*, \dots, \pi_H^*}(s_2) - V_2^{\pi_2, \dots, \pi_H}(s_2)] + 2\epsilon \\
&\leq \dots \\
&\leq 2H\epsilon
\end{aligned}$$

where the first step comes from definition of value function; the second step comes from Eq (1); the third step comes from optimality of  $\pi_1$ ; the fourth step comes from Eq (1); the fifth step comes from Bellman equation.  $\square$



#### 523 A.4 Neural network recovery

524 This section considers recovering neural network  $\langle v, \sigma(Wx) \rangle$  from the following two models:

- 525 • Noisy samples from

$$x \sim \mathcal{N}^{\leq B}(0, I_d), \quad y = \langle v, \sigma(Wx) \rangle + \xi \quad (2)$$

526 where  $\xi$  is  $\vartheta$  sub-Gaussian noise.

- 527 • Noiseless samples from

$$x \sim \mathcal{N}^{\leq B}(0, I_d), \quad y = \langle v, \sigma(Wx) \rangle \quad (3)$$

528 We use  $\mathcal{N}^{\leq B}(0, I_d)$  to denote the following distribution, to sample from  $\mathcal{N}^{\leq B}(0, I_d)$ , first sampling  
 529 from standard Gaussian  $\mathcal{N}(0, I_d)$  and then discard the samples that  $\|x\|_2^2 < B$ . Recall that  $B =$   
 530  $d \cdot \text{poly}(\log(d))$ . We consider more general homogeneous activation functions, specified by the  
 531 assumption that follow. This section mainly follows Zhong et al. [2017].

532 **Assumption A.1** (Property 3.1 of Zhong et al. [2017]). Assume  $\sigma'(x)$  is nonnegative and homoge-  
 533 neously bounded, i.e.  $0 \leq \sigma'(x) \leq L_1|x|^p$  for some constants  $L_1 > 0$  and  $p \geq 0$ .

534 **Definition A.2** (Part of property 3.2 of Zhong et al. [2017]). Define  $\rho(\sigma) := \min\{\beta_0(\sigma) - \alpha_0^2(\sigma) -$   
 535  $\sigma_1^2(\sigma), \beta_2(\sigma) - \alpha_1^2(\sigma) - \alpha_2^2(\sigma), \alpha_0(\sigma)\alpha_2(\sigma) - \alpha_1^2(\sigma)\}$ , where  $\alpha_q(\sigma) := \mathbb{E}_{z \sim \mathcal{N}(0,1)}[\phi'(\sigma z)z^q]$ ,  $q \in$   
 536  $\{0, 1, 2\}$ , and  $\beta_q(\sigma) := \mathbb{E}_{z \sim \mathcal{N}(0,1)}[(\phi')^2(\sigma z)z^q]$ .

537 **Assumption A.3** (Part of property 3.2 of Zhong et al. [2017]). The first derivative  $\sigma'(x)$  satisfies  
 538 that, for all  $z > 0$ , we have  $\rho(z) > 0$ .

539 **Assumption A.4** (Property 3.3 of Zhong et al. [2017]). The second derivative  $\sigma''(x)$  is either **(a)**  
 540 globally bounded or **(b)**  $\sigma''(x) = 0$  except for finite points.

541 Notice that ReLU, squared ReLU, leaky ReLU, and polynomial activation function functions all  
 542 satisfies the above assumption. We make the following assumption on the dimension of feature  
 543 vectors, which corresponds to how well algorithms can extract information about neural networks  
 544 from samples.

545 **Assumption A.5** (Rich feature). Assume  $d \geq \Omega(\log(\|W\|/\epsilon))$ .

546 Now following Zhong et al. [2017], we define some moments. First we introduce a notation.

**Definition A.6.** Define outer product  $\tilde{\otimes}$  as follows. For a vector  $v \in \mathbb{R}^d$  and an identity matrix  
 $I \in \mathbb{R}^{d \times d}$ ,

$$v \tilde{\otimes} I = \sum_{j=1}^d [v \otimes e_i \otimes e_j + e_j \otimes v \otimes e_j + e_j \otimes e_j \otimes v].$$

For a symmetric rank- $r$  matrix  $M = \sum_{i=1}^r s_i v_i v_i^\top$  and an identity matrix  $I \in \mathbb{R}^{d \times d}$ ,

$$M \tilde{\otimes} I = \sum_{i=1}^r s_i \sum_{j=1}^d \sum_{l=1}^6 A_{l,i,j}$$

547 where  $A_{1,i,j} = v_i \otimes v_i \otimes e_j \otimes e_j$ ,  $A_{2,i,j} = v_i \otimes e_j \otimes v_i \otimes e_j$ ,  $A_{3,i,j} = e_j \otimes v_i \otimes v_i \otimes e_j$ ,  
 548  $A_{4,i,j} = v_i \otimes e_j \otimes e_j \otimes v_i$ ,  $A_{5,i,j} = e_i \otimes v_i \otimes e_j \otimes v_i$ ,  $A_{6,i,j} = e_j \otimes e_j \otimes v_i \otimes v_i$ .

549 **Definition A.7.** Define  $M_1, M_2, M_3, M_4, m_{1,i}, m_{2,i}, m_{3,i}, m_{4,i}$  as follows:

$$\begin{aligned}
M_1 &:= \mathbb{E}[y \cdot n] \\
M_2 &:= \mathbb{E}[y \cdot x \otimes x - I] \\
M_3 &:= \mathbb{E}[y \cdot (x^{\otimes 3} - x \tilde{\otimes} I)] \\
M_4 &:= \mathbb{E}[y \cdot (x^{\otimes 4} - (x \otimes x) \tilde{\otimes} I + I \tilde{\otimes} I)] \\
\gamma_j(x) &:= \mathbb{E}_{z \sim \mathcal{N}(0,1)}[\sigma(x \cdot z) z^j], \forall j \in 0, 1, 2, 3, 4 \\
m_{1,i} &:= \gamma_1(\|w_i\|) \\
m_{2,i} &:= \gamma_2(\|w_i\|) - \gamma_0(\|w_i\|) \\
m_{3,i} &:= \gamma_3(\|w_i\|) - 3\gamma_1(\|w_i\|) \\
m_{4,i} &:= \gamma_4(\|w_i\|) + 3\gamma_0(\|w_i\|) - 6\gamma_2(\|w_i\|).
\end{aligned}$$

550 **Remark A.8.** Notice that since activation is fixed,  $m_{j,i} = \text{poly}(B_W)$  for all  $i \in [4]$  and  $i \in [k]$ .

551 **Assumption A.9** (Assumption 5.3 of Zhong et al. [2017]). Assume the activation function satisfies  
552 the followings:

- 553 • If  $M_i \neq 0$ , then  $m_{j,i} \neq 0$  for all  $i \in [k]$ .
- 554 • At least one of  $M_3$  and  $M_4$  is not zero.
- 555 • If  $M_1 = M_3 = 0$ , then  $\sigma(z)$  is an even function.
- 556 • If  $M_2 = M_4 = 0$ , then  $\sigma(z)$  is an odd function.

557 Now we state the theoretical result that recovers neural networks from noisy data.

**Theorem A.10** (Neural network recovery from noisy data). *Let the activation function  $\sigma$  satisfies Assumption A.1 and Assumption A.9. Let  $\kappa$  be the condition number of  $W$ . Given  $n$  samples from Eq (2). For any  $t \geq 1$  and  $\epsilon \in (0, 1)$  such that Assumption A.5 holds, if sample complexity*

$$n \geq \epsilon^{-2} \cdot d \cdot \text{poly}(t, \kappa, k, \vartheta, \log d)$$

558 *then there exists an algorithm that takes  $\tilde{O}(nkd)$  time and outputs a matrix  $\widehat{W} \in \mathbb{R}^{k \times d}$  and a vector*  
559  *$\widehat{v} \in \mathbb{R}^d$  such that with probability at least  $1 - d^{-\Omega(t)}$ ,*

$$\|\widehat{W} - W\|_F \leq \epsilon \text{poly}(k, \kappa) \cdot \|W\|_F, \text{ and } \widehat{v} = v.$$

560 The algorithm and proof are shown in Appendix A.4.1. The following corollary is therefore straight-  
561 forward.

**Corollary A.11.** *In the same setting as Theorem A.10. Suppose  $\|W\|_F \leq B_W$  and Assumption A.5 holds. Given  $n$  samples from Eq (2). If sample complexity*

$$n \geq \epsilon^{-2} \cdot d \cdot \text{poly}(t, \kappa, k, \log d, B_W, B_\phi, \vartheta)$$

562 *then there exists an algorithm that takes  $\tilde{O}(nkd)$  time and outputs a matrix  $\widehat{W} \in \mathbb{R}^{k \times d}$  and a vector*  
563  *$\widehat{v} \in \mathbb{R}^d$  such that with probability at least  $1 - d^{-\Omega(t)}$ , for all  $\|x\|_2 \leq B_\phi$*

$$|\langle \widehat{v}, \sigma(\widehat{W}x) \rangle - \langle v, \sigma(Wx) \rangle| \leq \epsilon.$$

564 Now we state the theoretical result that precisely recovers neural networks from noiseless data. The  
565 proof and method are shown in Appendix A.4.2.

566 **Theorem A.12** (Exact neural network recovery from noiseless data). *Let the activation function*  
567 *satisfies Assumption A.1 and Assumption A.9, Assumption A.3 and Assumption A.4(b). Given  $n$*   
568 *samples from Eq (3). Suppose sample complexity*

$$n \geq d \cdot \text{poly}(\kappa, t, k, \lambda, \log d)$$

569 *then there exists an algorithm that output exact  $W$  and  $v$  with probability at least  $1 - d^{-\Omega(t)}$ .*

#### 570 A.4.1 Recover neural networks from noisy data

571 In this section we prove Theorem A.10. Denote  $W = [w_1, \dots, w_k]$  where  $w_i \in \mathbb{R}^d$  and  $\bar{w}_i =$   
572  $w_i / \|w_i\|_2$ .

573 **Definition A.13.** Given a vector  $\alpha \in \mathbb{R}^d$ . Define  $P_2 := M_{j_2}(I, I, \alpha, \alpha)$  where  $j_2 = \min\{j \geq 2 : M_j \neq 0\}$  and  $P_3 := M_{j_3}(I, I, I, \alpha, \dots, \alpha)$  where  $j_3 = \min\{j \geq 3 : M_j \neq 0\}$ .  
574

575 The method of moments is presented in Algorithm 6. There are three main steps. First it computes  
576 the span of the rows of  $W$ . By power method, Line 7 finds the top- $k$  eigenvalues of  $CI + \hat{P}_2$  and  
577  $CI - \hat{P}_2$ . It then picks the largest  $k$  eigenvalues from  $CI + \hat{P}_2$  and  $CI - \hat{P}_2$ , by invoking TOPK in  
578 Line 15. Finally it orthogonalizes the corresponding eigenvectors in Line 19 and finds an orthogonal  
579 matrix  $V$  in the subspace spanned by  $\{\bar{w}_1, \dots, \bar{w}_k\}$ .

580 In the second step, the algorithm forms third order tensor  $R_3 = P_s(V, V, V) \in \mathbb{R}^{k \times k \times k}$  and use  
581 tensor decomposition in Kuleshov et al. [2015] to find  $\hat{u}$  which estimates  $s_i V^\top \bar{w}_i$  with unknown  
582 signs. In the third step the algorithm recovers  $s, v$  and  $w_i, i \in [k]$ . Due to homogeneous activation  
583 function, we assume  $v_i \in \{\pm 1\}$  and  $m_{j,i} = c_j \|w_i\|^{p+1}$  for universal constants  $c_j$ . We define  $Q_1$  and  
584  $Q_2$  as follows.

$$Q_1 = M_{l_1}(I, \underbrace{\alpha, \dots, \alpha}_{(l_1-1) \text{ } \alpha\text{'s}}) = \sum_{i=1}^k v_i c_{l_1} \|w_i\|^{p+1} (\alpha^\top \bar{w}_i)^{l_1-1} \bar{w}_i, \quad (4)$$

$$Q_2 = M_{l_2}(V, V, \underbrace{\alpha, \dots, \alpha}_{(l_2-2) \text{ } \alpha\text{'s}}) = \sum_{i=1}^k v_i c_{l_2} \|w_i\|^{p+1} (\alpha^\top \bar{w}_i)^{l_2-2} (V^\top \bar{w}_i) (V^\top \bar{w}_i)^\top, \quad (5)$$

585 where  $l_1 \geq 1$  such that  $M_{l_1} \neq 0$  and  $l_2 \geq 2$  such that  $M_{l_2} \neq 0$  are specified later. Then consider the  
586 following linear system.

$$z^* = \arg \min_{z \in \mathbb{R}^k} \left\| \sum_{i=1}^k z_i s_i \bar{w}_i - Q_1 \right\|, \text{ and } r^* = \arg \min_{r \in \mathbb{R}^k} \left\| \sum_{i=1}^k r_i V^\top \bar{w}_i (V^\top \bar{w}_i^*)^\top - Q_2 \right\|_F. \quad (6)$$

587 The solutions of the above linear systems are

$$z_i^* = v_i s_i^{l_1} c_{l_1} \|w_i\|^{p+1} (\alpha^\top s_i \bar{w}_i)^{l_1-1}, \text{ and } r_i = v_i s_i^{l_2} c_{l_2} \|w_i\|^{p+1} (\alpha^\top s_i \bar{w}_i)^{l_2-2}.$$

588 Since  $\hat{u}$  estimates  $s_i V^\top \bar{w}_i$ , we approximate  $s_i \bar{w}_i$  by  $V \hat{u}_i$  and approximate  $Q_1$  and  $Q_2$  by their  
589 empirical versions  $\hat{Q}_1$  and  $\hat{Q}_2$  in Line 28. Then we can solve the following linear systems.

$$\hat{z} = \arg \min_{z \in \mathbb{R}^k} \left\| \sum_{i=1}^k z_i V \hat{u}_i - \hat{Q}_1 \right\|, \text{ and } \hat{r} = \arg \min_{r \in \mathbb{R}^k} \left\| \sum_{i=1}^k r_i \hat{u}_i \hat{u}_i^\top - \hat{Q}_2 \right\|_F. \quad (7)$$

590 In this position we can estimate the magnitude  $\|w_i\|$  by  $(|\hat{z}_i| / (c_{j_1} (\alpha^\top V \hat{u}_i)^{l_1-1}))^{1/(p+1)}$  and recover  
591  $v_i$  and  $s_i$  by the standard procedures in Zhong et al. [2017]:

- 592 1. If  $M_1 = M_3 = 0$ , we choose  $l_1 = l_2 = \min\{j \in \{2, 4\} | M_j \neq 0\}$ . Return  $v_i^{(0)} =$   
593  $\text{sign}(\hat{r}_i c_{l_2})$  and  $s_i^{(0)}$  being  $-1$  or  $1$ .
- 594 2. If  $M_2 = M_4 = 0$ , we choose  $l_1 = \min\{j \in \{1, 3\} | M_j \neq 0\}$ ,  $l_2 = 3$ . Return  $v_i^{(0)}$  being  $-1$   
595 or  $1$  and  $s_i^{(0)} = \text{sign}(v_i^{(0)} \hat{z}_i c_{l_1})$ .
- 596 3. Otherwise, we choose  $l_1 = \min\{j \in \{1, 3\} | M_j \neq 0\}$ ,  $l_2 = \min\{j \in \{2, 4\} | M_j \neq 0\}$ .  
597 Return  $v_i^{(0)} = \text{sign}(\hat{r}_i c_{l_2})$  and  $s_i^{(0)} = \text{sign}(v_i^{(0)} \hat{z}_i c_{l_1})$ .

598 Since Algorithm 6 carries out the same computation as Zhong et al. [2017], the time complexity is the  
599 same. The difference of sample complexity comes from the noise  $\xi$  in the model and the truncation  
600 of standard Gaussian. The proof entails bounding the error in estimating  $P_2$  in Line 4,  $R_3$  in Line 20  
601 and  $Q_1, Q_2$  in Line 28.

---

**Algorithm 6** Method of moments
 

---

```

1: Inputs:  $S = \{(x_i, y_i) : i \in [n]\}$ 
2: Choose  $\alpha$  to be a random unit vector
3: Partition  $S$  into  $S_1, S_2, S_3, S_4$  of equal size
4:  $\hat{P}_2 \leftarrow \mathbb{E}_{S_1}[P_2], C \leftarrow 3\|P_2\|, T \leftarrow$  sufficient large constant
5: Choose  $\hat{V}_1^{(0)}, \hat{V}_1^{(0)} \in \mathbb{R}^{d \times k}$  to be random matrices ▷ Estimate subspace  $V$ 
6: for  $t = 1, \dots, T$  do
7:    $\hat{V}_1^{(t)} \leftarrow \text{QR}(C\hat{V}_1^{(t-1)} + \hat{P}_2\hat{V}_1^{(t-1)}), \hat{V}_2^{(t)} \leftarrow \text{QR}(C\hat{V}_2^{(t-1)} - \hat{P}_2\hat{V}_2^{(t-1)})$ 
8: end for
9: for  $j = 1, 2$  do
10:    $\hat{V}_j^{(T)} \leftarrow [\hat{V}_{j,1}, \dots, \hat{V}_{j,k}]$ 
11:   for  $i \in [k]$  do
12:      $\lambda_{j,i} \leftarrow |\hat{V}_{j,i} \hat{P}_2 \hat{V}_{j,i}|$ 
13:   end for
14: end for
15:  $\pi_1, \pi_2, k_1, k_2 \leftarrow \text{TOPK}(\lambda, k)$ 
16: for  $j = 1, 2$  do
17:    $V_j \leftarrow [\hat{V}_{j,\pi_j(1)}, \dots, \hat{V}_{j,\pi_j(k_j)}]$ 
18: end for
19:  $\tilde{V}_2 \leftarrow \text{QR}((I - V_1 V_1^\top) V_2), V \leftarrow [V_1, \tilde{V}_2]$ 
20:  $\hat{R}_3 \leftarrow \mathbb{E}_{S_2}[P_3(V, V, V)], \{\hat{u}_i\}_{i \in [k]} \leftarrow \text{TENSORDECOMPOSITION}(\hat{R}_3)$  ▷ Learn  $s_i V^\top \bar{w}_i$ 
21: if  $M_1 = M_3 = 0$  then
22:    $l_1, l_2 = \min\{j \in \{2, 4\} : M_j \neq 0\}$ 
23: else if  $M_2 = M_4 = 0$  then
24:    $l_1 \leftarrow \min\{j \in \{1, 3\} : M_j \neq 0\}, l_2 \leftarrow 3$ 
25: else
26:    $l_1 \leftarrow \min\{j \in \{1, 3\} : M_j \neq 0\}, l_2 = \min\{j \in \{2, 4\} : M_j \neq 0\}$ 
27: end if
28:  $\hat{Q}_1 \leftarrow \mathbb{E}_{S_3}[Q_1], \hat{Q}_2 \leftarrow \mathbb{E}_{S_4}[Q_1]$ 
29:  $\hat{z} \leftarrow \arg \min_z \|\sum_{i=1}^k z_i V \hat{u}_i - \hat{Q}_1\|, \hat{r} \leftarrow \arg \min_r \|\sum_{i=1}^k r_i \hat{u}_i \hat{u}_i - \hat{Q}_2\|_F$ 
30: for  $i = 1, \dots, k$  do ▷ Learn parameters  $v, W$ 
31:    $v_i^{(0)} \leftarrow \text{sign}(\hat{r}_i c_{l_2}), s_i^{(0)} \leftarrow \text{sign}(v_i^{(0)} \hat{z}_i c_{l_1})$ 
32:    $w_i^{(0)} \leftarrow s_i^{(0)} (|\frac{\hat{z}_i}{c_{l_1}(\alpha^\top V \hat{u}_i)^{l_1-1}}|)^{1/(p+1)} V \hat{u}_i$ 
33: end for
34:  $W^{(0)} \leftarrow [w_1^{(0)}, \dots, w_k^{(0)}]$ 
35: Return  $v^{(0)}, W^{(0)}$ 

```

---

602 **Lemma A.14.** Let  $\hat{P}_2$  be computed in Line 4 of Algorithm 6 and  $P_2$  defined in Definition A.13.  
 603 Suppose  $m_0 = \min_{i \in [k]} \{|m_{j_2, i}|^2 (\bar{w}_i^\top \alpha)^{2(j_2-2)}\}$  and

$$|S| \gtrsim d \cdot \text{poly}(\kappa, t, \vartheta, \log d) / (\epsilon^2 m_0)$$

604 then with probability at least  $1 - d^{-\Omega(t)}$ ,

$$\|P_2 - \hat{P}_2\| \leq \epsilon \sum_{i=1}^k |v_i m_{j_2, i} (\bar{w}_i^\top \alpha)^{j_2-2}|.$$

605 *Proof.* It suffices to bound  $\|M_2 - \widehat{M}_2\|$ ,  $\|M_3(I, I, \alpha) - \widehat{M}_3(I, I, \alpha)\|$  and  $\|M_4(I, I, \alpha, \alpha) -$   
 606  $\widehat{M}_4(I, I, \alpha, \alpha)\|$ .

607 Specifically, we show that with probability at least  $1 - d^{-t}$ ,

$$\|M_2 - \widehat{M}_2\| \leq \epsilon \sum_{i=1}^k |v_i m_{2, i}|. \quad (8)$$

$$\|M_3(I, I, \alpha) - \widehat{M}_3(I, I, \alpha)\| \leq \epsilon \sum_{i=1}^k |v_i m_{3,i}(\bar{w}_i^\top \alpha)|. \quad (9)$$

$$\|M_4(I, I, \alpha, \alpha) - \widehat{M}_4(I, I, \alpha, \alpha)\| \leq \epsilon \sum_{i=1}^k |v_i m_{4,i}(\bar{w}_i^\top \alpha)^2|. \quad (10)$$

608 Recall that for sample  $(x_j, y_j) \in S$ ,  $y_j = \sum_{i=1}^k v_i \sigma(w_i^\top x_j) + \xi_j$  where  $\xi_j$  is independent of  $x_j$ .  
 609 Consider each component  $i \in [k]$ . Define  $C_i(x_j), B_i(x_j) \in \mathbb{R}^{d \times d}$  as follows:

$$\begin{aligned} & C_i(x_j) \\ &= \mathbb{1}_{\|x\| \leq B} (\sigma(w_i^\top x_j) + \xi_j) \cdot (x_j^{\otimes 4} - (x_j \otimes x_j) \tilde{\otimes} I + I \tilde{\otimes} I)(I, I, \alpha, \alpha) \\ &= \mathbb{1}_{\|x\| \leq B} (\sigma(w_i^\top x_j) + \xi_j) \cdot ((x^\top \alpha)^2 x^{\otimes 2} - (\alpha^\top x)^2 I - 2(\alpha^\top x)(x\alpha^\top + \alpha x^\top) - xx^\top + 2\alpha\alpha^\top + I). \end{aligned}$$

610 Define  $B_i(x_j) = (\sigma(w_i^\top x_j) + \xi_j) \cdot ((x^\top \alpha)^2 x^{\otimes 2} - (\alpha^\top x)^2 I - 2(\alpha^\top x)(x\alpha^\top + \alpha x^\top) - xx^\top + 2\alpha\alpha^\top + I) \in \mathbb{R}^{d \times d}$ . Then from Claim D.5 we have  $\mathbb{E}[B_i(x_j)] = m_{4,i}(\bar{w}_i^\top \alpha)^2 \bar{w}_i \bar{w}_i^\top$ . By Assumption A.1,

$$\begin{aligned} & \sigma(w_i^\top x_j) \cdot (x_j^{\otimes 4} - (x_j \otimes x_j) \tilde{\otimes} I + I \tilde{\otimes} I)(I, I, \alpha, \alpha) \\ & \lesssim |w_i^\top x_j|^{p+1} + |\phi(0)| \cdot ((x_j^\top \alpha)^2 \|x_j\|^2 + 1 + \|x_j\|^2 + (\alpha^\top x_j)^2) \\ & \leq |w_i|^{p+1} \cdot |x_j|^{p+5}, \end{aligned}$$

612 using Claim D.1 and  $B \geq d \cdot \text{poly}(\log(d))$  we have

$$\|\mathbb{E}[C_i(x_j)] - m_{4,i}(\bar{w}_i^\top \alpha)^2 \bar{w}_i \bar{w}_i^\top\| \leq \mathbb{E}[\mathbb{1}_{\|x\| \geq B} |w_i|^{p+1} \cdot |x_j|^{p+5}] \leq (\|w_i\|d)^{p+5} \cdot e^{-\Omega(d \log d)} \leq \epsilon.$$

613 Also,  $\frac{1}{2} |m_{4,i}(\bar{w}_i^\top \alpha)^2| \leq \|\mathbb{E}[C_i(x_j)]\| \leq 2|m_{4,i}(\bar{w}_i^\top \alpha)^2|$ .

614 For any constant  $t \geq 1$ , we have with probability  $1 - 1/(d^{4t})$ ,

$$\begin{aligned} \|C_i(x)\| & \lesssim (|w_i^\top x_j|^{p+1} + |\phi(0)| + |\xi_j|) \cdot ((x_j^\top \alpha)^2 \|x_j\|^2 + 1 + \|x_j\|^2 + (\alpha^\top x_j)^2) \\ & \lesssim (\|w_i\|^{p+1} + |\phi(0)| + \vartheta) d \text{poly}(\log d, t) \end{aligned}$$

615 where the first step comes from Assumption A.1 and the second step comes from Claim D.2 and  
 616 Claim D.3.

617 Using Claim D.4, we have

$$\begin{aligned} \|\mathbb{E}[C_i(x)^2]\| & \lesssim (\mathbb{E}[(\phi(w_i^\top x_j) + \xi_j)^4])^{1/2} (\mathbb{E}[(x_j^\top \alpha)^8])^{1/2} (\mathbb{E}[\|x_j\|^4])^{1/2} \\ & \lesssim (\|w_i\|^{p+1} + |\phi(0)| + \vartheta)^2 d. \end{aligned}$$

618 Furthermore we have,

$$\max_{\|a\|=1} (\mathbb{E}[(a^\top C_i(x_j) a)^2])^{1/2} \lesssim (\mathbb{E}[(\phi(w_i^\top x_j) + \xi_j)^4])^{1/4} \lesssim \|w_i\|^{p+1} + |\phi(0)| + \vartheta.$$

619 Then by Claim D.6, with probability at least  $1 - d^{-t}$ ,

$$\begin{aligned} & \left\| m_{4,i}(\bar{w}_i^\top \alpha)^2 \bar{w}_i \bar{w}_i^\top - \frac{1}{|S|} \sum_{x_j \in S} C_i(x_j) \right\| \\ & \leq \left\| m_{4,i}(\bar{w}_i^\top \alpha)^2 \bar{w}_i \bar{w}_i^\top - \mathbb{E}[C_i(x_j)] \right\| + \left\| \mathbb{E}[C_i(x_j)] - \frac{1}{|S|} \sum_{x_j \in S} C_i(x_j) \right\| \\ & \leq \epsilon |m_{4,i}(\bar{w}_i^\top \alpha)^2|. \end{aligned}$$

620 Summing up all components  $i \in [k]$ , we proved Eq (10). Eq (8) and Eq (9) can be shown similarly.

621  $\square$

622 **Lemma A.15.** Let  $V \in \mathbb{R}^{d \times k}$  be an orthogonal matrix. Let  $\widehat{R}_3$  be computed in Line 20 of Algorithm 6  
623 and  $R_3 = P_3(V, V, V)$ . Suppose  $m_0 = \min_{i \in [k]} \{|m_{j_3, i}|^2 (\bar{w}_i^\top \alpha)^{2(j_3-3)}\}$  and

$$|S| \gtrsim d \cdot \text{poly}(\kappa, t, \vartheta, \log d) / (\epsilon^2 m_0)$$

624 then with probability at least  $1 - d^{-\Omega(t)}$ ,

$$\|R_3 - \widehat{R}_3\| \leq \epsilon \sum_{i=1}^k |v_i m_{j_3, i} (\bar{w}_i^\top \alpha)^{j_3-3}|.$$

625 *Proof.* From the definition of  $R_3$ , it suffices to bound  $\|M_3(V, V, V) - \widehat{M}_3(V, V, V)\|$  and  
626  $\|M_4(V, V, V, \alpha) - \widehat{M}_4(V, V, V, \alpha)\|$ .

627 Specifically, we show that with probability at least  $1 - d^{-t}$ ,

$$\|M_3(V, V, V) - \widehat{M}_3(V, V, V)\| \leq \epsilon \sum_{i=1}^k |v_i m_{3, i}|. \quad (11)$$

$$\|M_4(V, V, V, \alpha) - \widehat{M}_4(V, V, V, \alpha)\| \leq \epsilon \sum_{i=1}^k |v_i m_{4, i} (\bar{w}_i^\top \alpha)|. \quad (12)$$

628 Recall that for sample  $(x_j, y_j) \in S$ ,  $y_j = \sum_{i=1}^k v_i \sigma(w_i^\top x_j) + \xi_j$  where  $\xi_j$  is independent of  $x_j$ .  
629 Consider each component  $i \in [k]$ . Define  $T_i(x_j), S_i(x_j) \in \mathbb{R}^{k \times k \times k}$ :

$$\begin{aligned} T_i(x_j) &= (\sigma(w_i^\top x_j) + \xi_j) \cdot (x_i^\top \alpha \cdot v(x)^{\otimes 3} - (V^\top \alpha) \widetilde{\otimes} (v(x) \otimes v(x)) - \alpha^\top x \cdot v(x) \widetilde{\otimes} I + (V^\top \alpha) \widetilde{\otimes} I), \\ S_i(x_j) &= \mathbb{1}_{\|x\| \leq B} (\sigma(w_i^\top x_j) + \xi_j) \cdot \left( x_i^\top \alpha \cdot v(x)^{\otimes 3} - (V^\top \alpha) \widetilde{\otimes} (v(x) \otimes v(x)) \right. \\ &\quad \left. - \alpha^\top x \cdot v(x) \widetilde{\otimes} I + (V^\top \alpha) \widetilde{\otimes} I \right), \end{aligned}$$

630 where  $v(x) = V^\top x$ . Flatten  $T_i(x_j)$  along the first dimension to obtain  $B_i(x_j) \in \mathbb{R}^{k \times k^2}$ , flatten  
631  $S_i(x_j)$  along the first dimension to obtain  $C_i(x_j) \in \mathbb{R}^{k \times k^2}$ .

632 From Claim D.7,  $\mathbb{E}[B_i(x_j)] = m_{4, i} (\alpha^\top \bar{w}_i) (V^\top \bar{w}_i) \text{vec}((V^\top \bar{w}_i) (V^\top \bar{w}_i)^\top)^\top$ . Therefore we have,

$$\|\mathbb{E}[B_i(x)]\| = |m_{4, i} (\alpha^\top \bar{w}_i)| \cdot \|V^\top \bar{w}_i\|^3.$$

633 By Assumption A.1,

$$\begin{aligned} \|B_i(x)\| &\lesssim (|w_i^\top x_j|^{p+1} + |\phi(0)| + |\xi_j|) \cdot ((x_j^\top \alpha)^2 \|V^\top x_j\|^3 \\ &\quad + 3 \|V^\top x_j\|^3 + 3 |x_j^\top \alpha| \|V^\top x_j\| \sqrt{k} + 3 \|V^\top \alpha\| \sqrt{k}) \\ &\lesssim B_W^{p+1} \cdot \|x_j\|^{p+6}, \end{aligned}$$

634 using Claim D.1 and  $B \geq d \cdot \text{poly} \log(d)$ ,

$$\|\mathbb{E}[C_i(x_j)] - m_{4, i} (\alpha^\top \bar{w}_i) (V^\top \bar{w}_i) \text{vec}((V^\top \bar{w}_i) (V^\top \bar{w}_i)^\top)^\top\| \lesssim \mathbb{E}[\mathbb{1}_{\|x\| \leq B} \|w_i\|^{p+1} \cdot \|x_j\|^{p+6}] \leq \epsilon.$$

635 For any constant  $t \geq 1$ , we have with probability  $1 - d^{-\Omega(t)}$ ,

$$\begin{aligned} \|C_i(x)\| &\lesssim (|w_i^\top x_j|^{p+1} + |\phi(0)| + |\xi_j|) \cdot ((x_j^\top \alpha)^2 \|V^\top x_j\|^3 \\ &\quad + 3 \|V^\top x_j\|^3 + 3 |x_j^\top \alpha| \|V^\top x_j\| \sqrt{k} + 3 \|V^\top \alpha\| \sqrt{k}) \\ &\lesssim (\|w_i\|^{p+1} + |\phi(0)| + \vartheta) k^{3/2} \text{poly}(\log d, t) \end{aligned}$$

636 where the first step comes from Assumption A.1 and the second step comes from Claim D.2 and  
637 Claim D.3.

Using Claim D.4, we have

$$\begin{aligned} \|\mathbb{E}[C_i(x)C_i(x)^\top]\| &\lesssim (\mathbb{E}[(\phi(w_i^\top x_j) + \xi_j)^4])^{1/2} (\mathbb{E}[(\alpha^\top x_j)^4])^{1/2} (\mathbb{E}[\|V^\top x_j\|^6])^{1/2} \\ &\lesssim (\|w_i\|^{p+1} + |\phi(0)| + \vartheta)^2 k^{3/2}. \end{aligned}$$

ans

$$\begin{aligned} &\|\mathbb{E}[C_i(x)^\top C_i(x)]\| \\ &\lesssim (\mathbb{E}[(\phi(w_i^\top x_j) + \xi_j)^4])^{1/2} (\mathbb{E}[(\alpha^\top x_j)^4])^{1/2} (\mathbb{E}[\|V^\top x_j\|^4])^{1/2} \\ &\quad \cdot \left( \max_{\|A\|_F=1} \mathbb{E}[\langle A, (V^\top x_j)(V^\top x_j)^\top \rangle^4] \right)^{1/2} \\ &\lesssim (\|w_i\|^{p+1} + |\phi(0)| + \vartheta)^2 k^2. \end{aligned}$$

Furthermore we have,

$$\begin{aligned} &\max_{\|a\|=\|b\|=1} (\mathbb{E}[(a^\top C_i(x_j)b)^2])^{1/2} \\ &\lesssim (\mathbb{E}[(\phi(w_i^\top x_j) + \xi_j)^4])^{1/4} (\mathbb{E}[(\alpha^\top x_j)^4])^{1/4} \max_{\|a\|=1} (\mathbb{E}[(a^\top V^\top x_j)^4])^{1/2} \\ &\quad \cdot \max_{\|A\|_F=1} (\mathbb{E}[\langle A, (V^\top x_j)(V^\top x_j)^\top \rangle^4])^{1/2} \\ &\lesssim (\|w_i\|^{p+1} + |\phi(0)| + \vartheta)k. \end{aligned}$$

Then by Claim D.6, with probability at least  $1 - d^{-t}$ ,

$$\begin{aligned} &\left\| m_{4,i}(\alpha^\top \bar{w}_i)(V^\top \bar{w}_i) \text{vec}((V^\top \bar{w}_i)(V^\top \bar{w}_i)^\top)^\top - \frac{1}{|S|} \sum_{x_j \in S} C_i(x_j) \right\| \\ &\leq \left\| m_{4,i}(\alpha^\top \bar{w}_i)(V^\top \bar{w}_i) \text{vec}((V^\top \bar{w}_i)(V^\top \bar{w}_i)^\top)^\top - \mathbb{E}[C_i(x_j)] \right\| + \left\| \mathbb{E}[C_i(x_j)] - \frac{1}{|S|} \sum_{x_j \in S} C_i(x_j) \right\| \\ &\leq \epsilon |v_i m_{4,i}(\bar{w}_i^\top \alpha)|. \end{aligned}$$

Summing up all neurons  $i \in [k]$ , we proved Eq (12). Eq (11) can be shown similarly.

□

**Lemma A.16.** Let  $\hat{Q}_1$  and  $\hat{Q}_2$  be computed in Line 28 of Algorithm 6. Let  $Q_1$  be defined by Eq 4 and  $Q_2$  be defined by Eq 5. Suppose  $m_0 = \min_{i \in [k]} \{|m_{j_1,i}|^2 (\bar{w}_i^\top \alpha)^{2(j_1-1)}, |m_{j_2,i}|^2 (\bar{w}_i^\top \alpha)^{2(j_2-2)}\}$  and

$$|S| \gtrsim d \cdot \text{poly}(\kappa, t, \vartheta, \log d) / (\epsilon^2 m_0)$$

then with probability at least  $1 - d^{-\Omega(t)}$ ,

$$\begin{aligned} \|Q_1 - \hat{Q}_1\| &\leq \epsilon \sum_{i=1}^k |v_i m_{j_1,i} (\bar{w}_i^\top \alpha)^{j_1-1}|, \\ \|Q_2 - \hat{Q}_2\| &\leq \epsilon \sum_{i=1}^k |v_i m_{j_2,i} (\bar{w}_i^\top \alpha)^{j_2-2}|. \end{aligned}$$

*Proof.* Recall the expression of  $Q_1$  and  $Q_2$ ,

$$\begin{aligned} Q_1 &= M_{I_1}(I, \underbrace{\alpha, \dots, \alpha}_{(j_1-1) \text{ } \alpha\text{'s}}) = \sum_{i=1}^k v_i c_{j_1} \|w_i\|^{p+1} (\alpha^\top \bar{w}_i)^{j_1-1} \bar{w}_i, \\ Q_2 &= M_{j_2}(V, V, \underbrace{\alpha, \dots, \alpha}_{(j_2-2) \text{ } \alpha\text{'s}}) = \sum_{i=1}^k v_i c_{j_2} \|w_i\|^{p+1} (\alpha^\top \bar{w}_i)^{j_2-2} (V^\top \bar{w}_i)(V^\top \bar{w}_i)^\top. \end{aligned}$$

The proof is essentially similar to Lemma A.14 and Lemma A.15.

□

649 We also use the following Lemmata from Zhong et al. [2017].

650 **Lemma A.17** (Lemma E.6 of Zhong et al. [2017]). *Let  $P_2$  be defined as in Definition. A.13 and*  
651  *$\hat{P}_2$  be its empirical version calculated in Line 4 of Algorithm 6. Let  $U \in \mathbb{R}^{d \times k}$  be the orthogonal*  
652 *column span of  $W \in \mathbb{R}^{d \times k}$ . Assume  $\|\hat{P}_2 - P_2\| \leq \sigma_k(P_2)/10$ . Let  $C$  be a large enough positive*  
653 *number such that  $C > 2\|P_2\|$ . Then after  $T = O(\log(1/\epsilon))$  iterations, the  $V \in \mathbb{R}^{d \times k}$  computed in*  
654 *Algorithm 6 will satisfy*

$$\|UU^\top - VV^\top\| \lesssim \|\hat{P}_2 - P_2\|/s_k(P_2) + \epsilon,$$

655 which implies

$$\|(I - VV^\top)w_i\| \lesssim (\|\hat{P}_2 - P_2\|/s_k(P_2) + \epsilon)\|w_i\|.$$

656 **Lemma A.18** (Lemma E.11 in Zhong et al. [2017]). *Given two matrices  $A, \tilde{A} \in \mathbb{R}^{d \times k}$ , and two*  
657 *vectors  $b, \tilde{b} \in \mathbb{R}^d$ . Let  $z^* = \arg \min_{z \in \mathbb{R}^k} \|Az - b\|$  and  $\hat{z} = \arg \min_{z \in \mathbb{R}^k} \|(A + \tilde{A})z - (b + \tilde{b})\|$ . If*  
658  *$\|\tilde{A}\| \leq \frac{1}{4\kappa}\sigma_k(A)$  and  $\|\tilde{b}\| \leq \frac{1}{4}\|b\|$ , then, we have*

$$\|z^* - \hat{z}\| \lesssim (s_k^{-4}(A)s_1^2(A) + s_k^{-2}(A))\|b\|\|\tilde{A}\| + s_k^{-2}(A)s_1(A)\|\tilde{b}\|.$$

659 **Lemma A.19** (Lemma E.13 in Zhong et al. [2017]). *Let  $U \in \mathbb{R}^{d \times k}$  be the orthogonal column span of*  
660  *$W^*$ . Let  $V \in \mathbb{R}^{d \times k}$  denote an orthogonal matrix satisfying that  $\|VV^\top - UU^\top\| \leq \hat{\delta}_2 \lesssim 1/(\kappa^2\sqrt{k})$ .*  
661 *For each  $i \in [k]$ , let  $\hat{u}_i$  denote the vector satisfying  $\|\hat{u}_i - V^\top \bar{w}_i\| \leq \hat{\delta}_3 \lesssim 1/(\kappa^2\sqrt{k})$ . Let  $Q_1$  be*  
662 *defined as in Eq. (4) and  $\hat{Q}_1$  be the empirical version of  $Q_1$  such that  $\|Q_1 - \hat{Q}_1\| \leq \hat{\delta}_4\|Q_1\| \leq$*   
663  *$\frac{1}{4}\|Q_1\|$ .*

664 *Let  $z^* \in \mathbb{R}^k$  and  $\hat{z} \in \mathbb{R}^k$  be defined as in Eq. (6) and Eq. (7). Then*

$$|\hat{z}_i - z_i^*| \leq (\kappa^4 k^{3/2}(\hat{\delta}_2 + \hat{\delta}_3) + \kappa^2 k^{1/2} \hat{\delta}_4)\|z^*\|_1.$$

665 **Lemma A.20** (Lemma E.14 in Zhong et al. [2017]). *Let  $U \in \mathbb{R}^{d \times k}$  be the orthogonal column span*  
666 *of  $W^*$  denote an orthogonal matrix satisfying that  $\|VV^\top - UU^\top\| \leq \hat{\delta}_2 \lesssim 1/(\kappa\sqrt{k})$ . For each*  
667  *$i \in [k]$ , let  $\hat{u}_i$  denote the vector satisfying  $\|\hat{u}_i - V^\top \bar{w}_i^*\| \leq \hat{\delta}_3 \lesssim 1/(\sqrt{k}\kappa^3)$ . Let  $Q_2$  be defined*  
668 *as in Eq. (5) and  $\hat{Q}_2$  be the estimation of  $Q_2$  such that  $\|Q_2 - \hat{Q}_2\|_F \leq \hat{\delta}_4\|Q_2\|_F \leq \frac{1}{4}\|Q_2\|_F$ . Let*  
669  *$r^* \in \mathbb{R}^k$  and  $\hat{r} \in \mathbb{R}^k$  be defined as in Eq. (6) and Eq. (7). Then*

$$|\hat{r}_i - r_i^*| \leq (k^3 \kappa^8 \hat{\delta}_3 + \kappa^2 k^2 \hat{\delta}_4)\|r^*\|.$$

670 Now we are in the position of proving Theorem A.10.

671 *Proof.* Consider Algorithm 6. Using triangle inequality and  $V^\top V = I$  we have the following,

$$\begin{aligned} \|\bar{w}_i - s_i V \hat{u}_i\| &\leq \|VV^\top \bar{w}_i - \bar{w}_i\| + \|VV^\top \bar{w}_i - V s_i \hat{u}_i\| \\ &= \|VV^\top \bar{w}_i - \bar{w}_i\| + \|V^\top \bar{w}_i - s_i \hat{u}_i\|. \end{aligned} \quad (13)$$

672 For  $\|VV^\top \bar{w}_i - \bar{w}_i\|$ , we have

$$\begin{aligned} \|VV^\top \bar{w}_i - \bar{w}_i\| &\leq (\|\hat{P}_2 - P_2\|/s_k(P_2) + \epsilon) \\ &\leq (\text{poly}(k, \kappa)\|\hat{P}_2 - P_2\| + \epsilon) \\ &\leq \text{poly}(k, \kappa)\epsilon, \end{aligned} \quad (14)$$

673 where the first step follows by Lemma , the second step follows by  $\sigma_k(P_2) \geq 1/\text{poly}(k, \kappa)$ , and the  
674 last step follows by  $\|\hat{P}_2 - P_2\| \leq \epsilon \text{poly}(k, \kappa)$  if the number of samples is proportional to  $\tilde{O}(d/\epsilon^2)$   
675 as shown in Lemma A.14.

676 For  $\|V^\top \bar{w}_i - s_i \hat{u}_i\|$ , we have

$$\|V^\top \bar{w}_i - s_i \hat{u}_i\| \leq \text{poly}(k, \kappa)\|\hat{R}_3 - R_3\| \leq \epsilon \text{poly}(k, \kappa), \quad (15)$$



where the first step follows by Theorem 3 in Kuleshov et al. [2015] and the last step follows by Lemma A.15.

Plugging (14) and (15) into Eq. (13), we have

$$\|\bar{w}_i - s_i V \hat{u}_i\| \leq \epsilon \text{poly}(k, \kappa). \quad (16)$$

Next we bound the error in  $\hat{r}$  and  $\hat{z}$ . We have,

$$|\hat{r}_i - r_i^*| \leq \text{poly}(k, \kappa) \max\{\|Q_1 - \hat{Q}_1\|, \|Q_2 - \hat{Q}_2\|\} \cdot \|r^*\| \leq \epsilon \text{poly}(k, \kappa) \cdot \|r^*\| \quad (17)$$

where the first step comes from Lemma A.19 and the second step comes from Lemma A.16. Furthermore,

$$|\hat{z}_i - z_i^*| \leq \text{poly}(k, \kappa) \max\{\|Q_1 - \hat{Q}_1\|, \|Q_2 - \hat{Q}_2\|\} \cdot \|z^*\|_1 \leq \epsilon \text{poly}(k, \kappa) \|z^*\|_1, \quad (18)$$

where the first step comes from Lemma A.20 and the second step comes from Lemma A.16. Combining Eq (17), Eq (18) and Eq (16), the output in Line 32 satisfies  $\|w_i^{(0)} - w_i\|_F \leq \epsilon \text{poly}(k, \kappa) \cdot \|w_i\|_F$ . Since  $v_i$  are discrete values, they are exactly recovered.

□

#### A.4.2 Exact recovery of neural networks from noiseless data

In this section we prove Theorem A.12. Similar to Appendix A.4.1, denote  $W = [w_1, \dots, w_k]$  where  $w_i \in \mathbb{R}^d$  and  $\widehat{W} = [\widehat{w}_1, \dots, \widehat{w}_k]$ . We define the empirical loss and the population loss as follows,

$$L_n(\widehat{W}) = \frac{1}{2n} \sum_{i=1}^n \left( \sum_{i=1}^k v_i \sigma(\widehat{w}_i^\top x_i) - y_i \right)^2, \quad (19)$$

$$L(\widehat{W}) = \frac{1}{2} \mathbb{E} \left[ \left( \sum_{i=1}^k v_i \sigma(\widehat{w}_i^\top x) - y \right)^2 \right]. \quad (20)$$

**Definition A.21.** Let  $s_i$  be the  $i$ -th singular value of  $W$ ,  $\lambda := \prod_{i=1}^k (s_i/s_k)$ . Let  $\tau = (3s_1/2)^{4p} / \min_{z \in [s_k/2, 3s_1/2]} \{\rho^2(z)\}$ .

We use the follow results adapted from Zhong et al. [2017]. The only difference is that we use truncated Gaussian  $\mathcal{N}^{\leq B}(0, I_d)$ , and due to  $B = d \text{poly} \log(d)$  we can bound its difference between standard Gaussian in the same way as Appendix A.4.1.

**Lemma A.22** (Concentration, adapted from Lemma D.11 in Zhong et al. [2017]). *Let samples size  $n \geq \epsilon^{-2} d \tau \text{poly}(\log d, t)$ , then with probability at least  $1 - d^{-\Omega(t)}$ ,*

$$\|\nabla^2 L_n(W) - \nabla^2 L(W)\| \lesssim k \sigma_1^{2p} \epsilon \quad (21)$$

**Lemma A.23** (Adapted from Lemma D.16 in Zhong et al. [2017]). *Let  $\{x_1, \dots, x_n\}$  denote a set of samples from Distribution  $\mathcal{D}$ . Assume activation  $\sigma(\cdot)$  satisfies Assumption A.4 and Assumption A.3. Then for any  $t \geq 1$ , if  $n \geq d \text{poly}(\log d, t)$ , with probability at least  $1 - d^{-t}$ , for any  $\widehat{W}$  (which is not necessarily to be independent of samples) satisfying  $\|W - \widehat{W}\| \leq \sigma k/4$ , we have*

$$\|\nabla^2 L_n(\widehat{W}) - \nabla^2 L_n(W)\| \leq k s_1^p \|W - \widehat{W}\| d^{(p+1)/2}.$$

Now we prove Theorem A.12.

*Proof.* The exact recovery consists of first finding (exact)  $v$  and (approximate)  $\widehat{W}$  close enough to  $W$  by tensor method (Appendix A.4.1), and then minimizing the empirical loss  $L_n(\cdot)$ . We will prove that  $L_n(\cdot)$  is locally strongly convex, thus we find the precise  $W$ .

From Lemma D.3 from Zhong et al. [2017] we know:

$$\Omega(\rho(s_k)/\lambda)I \preceq \nabla^2 L(W) \preceq O(k s_1^{2p})I. \quad (22)$$

706 From Lemma A.22, we need  $n \geq \frac{k^2 \lambda^2 s_1^{4p}}{\rho^2(s_k)} d \tau \text{poly}(\log d, t)$  for  $\nabla^2 L_n(W)$  to be positive definite.

707 Next we uniformly bound Lipschitzness of  $\nabla^2 L_n$ . From Lemma A.23 there exists a universal constant  
 708  $c$ , for all  $\widehat{W}$  that satisfies  $\|W - \widehat{W}\| \leq c k s_1^{2p} / (k s_1^p d^{(p+1)/2}) = c s_1^p d^{-(p+1)/2}$ ,  $\nabla L_n^2(\widehat{W}) \gtrsim k s_1^{2p}$   
 709 uniformly. So there is a unique minimizer of  $L_n$  in this region.

710 Notice  $L_n(W) = 0$ , therefore we can find  $W$  by directly minimizing the empirical loss as long as  
 711 we find any  $\widehat{W}$  in this region. This can be achieved by tensor method in Appendix A.4.1. We thus  
 712 complete the proof.

713 □

## 714 B Omitted Proofs in Section 5

715 For the proofs of Theorem 5.2, Example 5.3, and Example 5.4, we refer the readers to [Anonymous].

716 **Lemma B.1.** *Consider the polynomial family  $\mathcal{F}_V$  of dimension  $D$ . Assume that  $n > 2D$ . For any  
 717  $E \in \mathbb{R}^d$  that is of positive measure, by sampling  $n$  samples  $\{x_i\}$  i.i.d. from  $\mathbb{P}_{x \in \mathcal{N}(0, I_d)}(\cdot | x \in E)$  and  
 718 observing the noiseless feedbacks  $y_i = f^*(x_i)$ , one can almost surely uniquely determine the  $f^*$  by  
 719 solving the system of equations  $y_i = f(x_i)$ ,  $i = 1, \dots, n$ , for  $f \in \mathcal{F}_V$ .*

720 *Proof.* By Theorem 5.2, there exists a set  $N \in \mathbb{R}^d \times \dots \mathbb{R}^d$  of Lebesgue measure zero, such that if  
 721  $(x_1, \dots, x_n) \notin N$ , one can uniquely determine the  $f^*$  by the observations on the  $n$  samples. There-  
 722 fore, we only need to show that with probability 1, the sampling procedure returns  $(x_1, \dots, x_n) \notin N$ .  
 723 This is because

$$\begin{aligned} \mathbb{P}(x_1, \dots, x_n \in N) &= \mathbb{P}_{x_i \in \mathcal{N}(0, I_d)}((x_1, \dots, x_n) \in N \mid x_1, \dots, x_n \in E) \\ &= \frac{\mathbb{P}_{x_i \in \mathcal{N}(0, I_d)}((x_1, \dots, x_n) \in N \cap (E \times \dots \times E))}{\mathbb{P}_{x_i \in \mathcal{N}(0, I_d)}((x_1, \dots, x_n) \in (E \times \dots \times E))} \\ &= \frac{0}{[\mathbb{P}_{x_1 \in \mathcal{N}(0, I_d)}(x_1 \in E)]^n} \\ &= 0. \end{aligned}$$

724 □

725 By Lemma B.1 above, it is not hard to see that Algorithms 4 and 5 work.

## 726 C Omitted Constructions and Proofs in Subsection 5.1

727 **Construction of the Reward Functions** The following construction of the polynomial hard case is  
 728 adopted from [Anonymous].

729 Let  $d$  be the dimension of the feature space. Let  $e_i$  denotes the  $i$ -th standard orthonormal basis of  $\mathbb{R}^d$ ,  
 730 i.e.,  $e_i$  has only one 1 at the  $i$ -th entry and 0's for other entries. Let  $p$  denote the highest order of the  
 731 polynomial. We assume  $d \gg p$ . We use  $\Lambda$  to denote a subset of the  $p$ -th multi-indices

$$\Lambda = \{(\alpha_1, \dots, \alpha_p) \mid 1 \leq \alpha_1 \leq \dots \leq \alpha_p \leq d\}.$$

732 For an  $\alpha = (\alpha_1, \dots, \alpha_p) \in \Lambda$ , denote  $M_\alpha = e_{\alpha_1} \otimes \dots \otimes e_{\alpha_p}$ ,  $x_\alpha = e_{\alpha_1} + \dots + e_{\alpha_p}$ .

733 The model space  $\mathcal{M}$  is a subset of rank-1  $p$ -th order tensors, which is defined as  $\mathcal{M} = \{M_\alpha \mid \alpha \in \Lambda\}$ .  
 734 We define two subsets of feature space  $\mathcal{F}_0$  and  $\mathcal{F}$  as  $\mathcal{F}_0 = \{x_\alpha \mid \alpha \in \Lambda\}$ ,  $\mathcal{F} = \text{conv}(\mathcal{F}_0)$ . For  $M_\alpha \in$   
 735  $\mathcal{M}$ ,  $x \in \mathcal{F}$ , define  $r(M_\alpha, x)$  as  $r(M_\alpha, x) = \langle M_\alpha, x^{\otimes p} \rangle = \prod_{i=1}^p \langle e_{\alpha_i}, x \rangle$ . We assume that for each  
 736 level  $h$ , there is a  $M^{(h)} = M_{\alpha^{(h)}} \in \mathcal{M}$ , and the noiseless reward is  $r_h(s, a) = r(M^{(h)}, \phi_h(s, a))$ .

737 We have the following properties.

738 **Proposition C.1** (Anonymous). *For  $M_\alpha \in \mathcal{M}$  and  $x_{\alpha'} \in \mathcal{F}_0$ , we have*

$$r(M_\alpha, x_{\alpha'}) = \mathbb{I}_{\{\alpha = \alpha'\}}.$$

739 **Proposition C.2.** For  $M_\alpha \in \mathcal{M}$ , we have

$$\max_{x \in \mathcal{F}} r(M_\alpha, x) = 1.$$

740 *proof of Proposition C.2.* For all  $x \in \mathcal{F}$ , since  $\mathcal{F} = \text{conv}(\mathcal{F}_0)$ , we can write

$$x = \sum_{\alpha \in \Lambda} p_\alpha (e_{\alpha_1} + \cdots + e_{\alpha_p}),$$

741 where  $\sum_{\alpha \in \Lambda} p_\alpha = 1$  and  $p_\alpha \geq 0$ . Therefore,

$$r(M_{\alpha'}, x) = \prod_{i=1}^p \langle e_{\alpha'_i}, x \rangle.$$

742 Plug in the expression of  $x$ , we have

$$\begin{aligned} \langle e_{\alpha'_i}, x \rangle &= \sum_{\alpha} p_\alpha \langle e_{\alpha'_i}, e_{\alpha_1} + \cdots + e_{\alpha_p} \rangle \\ &= \sum_{\alpha} p_\alpha \mathbb{I}_{\{\alpha'_i \in \alpha\}} \\ &\leq \sum_{\alpha} p_\alpha = 1. \end{aligned}$$

743 Therefore,

$$\begin{aligned} r(M_{\alpha'}, x) &= \prod_{i=1}^p \langle e_{\alpha'_i}, x \rangle \\ &= \left( \sum_{\alpha} p_\alpha \mathbb{I}_{\{\alpha'_1 \in \alpha\}} \right) \cdots \left( \sum_{\alpha} p_\alpha \mathbb{I}_{\{\alpha'_p \in \alpha\}} \right) \\ &\leq 1. \end{aligned}$$

744 Finally, since  $r(M_{\alpha'}, x_{\alpha'}) = 1$ , we have  $\max_{x \in \mathcal{F}} r(M_\alpha, x) = 1$ .  $\square$

745 **MDP constructions** Consider a family of MDPs with only two states  $\mathcal{S} = \{S_{\text{good}}, S_{\text{bad}}\}$ . The  
746 action set  $\mathcal{A}$  is set to be  $\mathcal{F}$ . Let  $f$  be a mapping from  $\mathcal{F}$  to  $\mathcal{F}_0$  such that  $f$  is identity when restricted  
747 to  $\mathcal{F}_0$ . For all level  $h \in [H]$ , we define the feature map  $\phi_h : \mathcal{S} \times \mathcal{A} \rightarrow \mathcal{F}$  to be

$$\phi_h(s, a) = \begin{cases} a & \text{if } s = S_{\text{good}}, \\ f(a) & \text{if } s = S_{\text{bad}}. \end{cases}$$

748 Given an unknown sequence of indices  $\alpha^{(1)}, \dots, \alpha^{(H)}$ , the reward function at level  $h$  is  $r_h(s, a) =$   
749  $r(M_{\alpha^{(h)}}, \phi_h(s, a))$ . Specifically, we have

$$r_h(S_{\text{good}}, a) = r(M_{\alpha^{(h)}}, a), \quad r_h(S_{\text{bad}}, a) = r(M_{\alpha^{(h)}}, f(a)).$$

750 The transition  $P_h$  is constructed as

$$P_h(S_{\text{bad}} | s, a) = 1 \text{ for all } s \in \mathcal{S}, a \in \mathcal{A}.$$

751 This construction means it is impossible for the online scenarios to reach the good state for  $h > 1$ .

752 The next proposition shows that  $Q_h^*$  is polynomial realizable and falls into the case of Example 5.4.

753 **Proposition C.3.** We have for all  $h \in [H]$  and  $s \in \mathcal{S}$ ,  $a \in \mathcal{A}$ ,  $V_h^*(s) = H - h + 1$  and  $Q_h^*(s, a) =$   
754  $r_h(s, a) + H - h + 1$ . Furthermore,  $Q_h^*(s, a)$ , viewed as the function of  $\phi_h(s, a)$ , is a polynomial of  
755 the form  $q_h(U_h \phi_h(s, a))$  for some degree- $p$  polynomial  $q_h$  and  $U_h \in \mathbb{R}^{p \times d}$ .

756 *proof of Proposition C.3.* First notice that by Proposition C.2, for all  $h \in [H]$  and  $s \in \mathcal{S}$ , we have

$$\max_{a \in \mathcal{A}} r_h(s, a) = 1.$$

Therefore, by induction, suppose we have proved for all  $s'$ ,  $V_{h+1}^*(s') = H - h$ , then we have

$$\begin{aligned} V_h^*(s) &= \max_{a \in \mathcal{A}} Q_h^*(s, a) \\ &= \max_{a \in \mathcal{A}} \{r_h(s, a) + \mathbb{E}_{s' \sim P_h(\cdot|s, a)}[V_{h+1}^*(s')]\} \\ &= 1 + H - h. \end{aligned}$$

Then we have  $Q_h^*(s, a) = r_h(s, a) + H - h + 1$ .

Furthermore, we have

$$\begin{aligned} Q_h^*(s, a) &= r_h(s, a) + H - h + 1 \\ &= r(M_{\alpha^{(h)}}, \phi_h(s, a)) + H - h + 1 \\ &= \prod_{i=1}^p \langle e_{\alpha_i^{(h)}}, \phi_h(s, a) \rangle + H - h + 1 \\ &= q_h(U_h \phi_h(s, a)), \end{aligned}$$

where  $q_h(x_1, \dots, x_p) = x_1 x_2 \cdots x_p + (H - h + 1)$  and  $U_h \in \mathbb{R}^{p \times d}$  is a matrix with  $e_{\alpha_i^{(h)}}$  as the  $i$ -th row.  $\square$

**Theorem C.4.** Under the online RL setting, any algorithm needs to play at least  $\binom{d}{p} - 1 = \Omega(d^p)$  episodes to identify  $\alpha^{(2)}, \dots, \alpha^{(H)}$  and thus to identify the optimal policy.

*proof of Theorem C.4.* Under the online RL setting, any algorithm enters and remains in  $S_{\text{bad}}$  for  $h > 1$ . When  $s_h = S_{\text{bad}}$ , no matter what  $a_h$  the algorithm chooses, we have  $\phi_h(s_h, a_h) = f(a_h) \in \mathcal{F}_0$ . Notice that for any  $M_{\alpha^{(h)}} \in \mathcal{M}$  and any  $x_\alpha \in \mathcal{F}_0$ , we have  $r(M_{\alpha^{(h)}}, x_\alpha) = \mathbb{I}_{\{\alpha = \alpha^{(h)}\}}$  as Proposition C.1 suggests. Hence, we need to play  $\binom{d}{p} - 1$  times at level  $h$  in the worst case to find out  $\alpha^{(h)}$ . The argument holds for all  $h = 2, 3, \dots, H$ .  $\square$

**Theorem C.5.** Under the generative model setting, by querying  $2d(p+1)^p H = O(dH)$  samples, we can almost surely identify  $\alpha^{(1)}, \alpha^{(2)}, \dots, \alpha^{(H)}$  and thus identify the optimal policy.

*proof of Theorem C.5.* By Proposition C.3, we know that  $Q_h^*(s, a)$ , viewed as the function of  $\phi_h(s, a)$ , falls into the case of Example 5.4 with  $k = p$ .

Next, notice that for all  $h \in [H]$ ,  $\{\phi_h(s, a) \mid s \in \mathcal{S}, a \in \mathcal{A}\} = \mathcal{F}$ . Although  $\mathcal{F}$  is not of positive measure, we can actually know the value of  $Q_h^*$  when  $\phi_h(s, a)$  is in  $\text{conv}(\mathcal{F}, \mathbf{0})$  since the reward is  $p$ -homogenous. Specifically, for every feature of the form  $c \cdot \phi_h(s, a)$ , where  $0 \leq c \leq 1$  and  $\phi_h(s, a) \in \mathcal{F}$ , the reward is  $c^p$  times the reward of  $(s, a)$ . Therefore, to get the reward at  $c \cdot \phi_h(s, a)$ , we only need to query the generative model at  $(s, a)$  of level  $h$ , and then multiply the reward by  $c^p$ .

Notice that  $\text{conv}(\mathcal{F}, \mathbf{0})$  is of positive Lebesgue measure. By Theorem 5.7, we know that only  $2d(p+1)^p H = O(dH)$  samples are needed to determine the optimal policy almost surely.

$\square$

## D Technical claims

**Claim D.1.** Let  $\chi^2(d)$  denote  $\chi^2$ -distribution with freedom  $d$ . For any  $t > 0$  we have,

$$\Pr_{z \sim \chi^2(d)}(z \geq d + 2t + 2\sqrt{dt}) \leq e^{-t}$$

We use the following facts from Zhong et al. [2017].

**Claim D.2.** Given a fixed vector  $z \in \mathbb{R}^d$ , for any  $C \geq 1$  and  $n \geq 1$ , we have

$$\Pr_{x \sim \mathcal{N}(0, I_d)}[|\langle x, z \rangle|^2 \leq 5C\|z\|^2 \log n] \geq 1 - 1/(nd^C).$$

785 **Claim D.3.** For any  $C \geq 1$  and  $n \geq 1$ , we have

$$\Pr_{x \sim \mathcal{N}(0, I_d)} [\|x\|^2 \leq 5Cd \log n] \geq 1 - 1/(nd^C).$$

786 **Claim D.4.** Let  $a, b, c \geq 0$  be three constants, let  $u, v, w \in \mathbb{R}^d$  be three vectors, we have

$$\mathbb{E}_{x \sim \mathcal{N}(0, I_d)} [|u^\top x|^a |v^\top x|^b |w^\top x|^c] \approx \|u\|^a \|v\|^b \|w\|^c.$$

787 **Claim D.5.** For each  $j \in [4]$ ,  $M_j = \sum_{i=1}^k v_i^* m_{j,i} \bar{w}_i^{*\otimes j}$ .

788 **Claim D.6.** Let  $\mathcal{B}$  denote a distribution over  $\mathbb{R}^{d_1 \times d_2}$ . Let  $d = d_1 + d_2$ . Let  $B_1, B_2, \dots, B_n$  be  
789 i.i.d. random matrices sampled from  $\mathcal{B}$ . Let  $\bar{B} = \mathbb{E}_{B \sim \mathcal{B}}[B]$  and  $\hat{B} = \frac{1}{n} \sum_{i=1}^n B_i$ . For parameters  
790  $m \geq 0, \gamma \in (0, 1), \nu > 0, L > 0$ , if the distribution  $\mathcal{B}$  satisfies the following four properties,

- (1)  $\Pr_{B \sim \mathcal{B}} [\|B\| \leq m] \geq 1 - \gamma;$
- (2)  $\left\| \mathbb{E}_{B \sim \mathcal{B}}[B] \right\| > 0;$
- (3)  $\max \left( \left\| \mathbb{E}_{B \sim \mathcal{B}}[BB^\top] \right\|, \left\| \mathbb{E}_{B \sim \mathcal{B}}[B^\top B] \right\| \right) \leq \nu;$
- (4)  $\max_{\|a\|=\|b\|=1} \left( \mathbb{E}_{B \sim \mathcal{B}} \left[ (a^\top B b)^2 \right] \right)^{1/2} \leq L.$

791 Then we have for any  $0 < \epsilon < 1$  and  $t \geq 1$ , if

$$n \geq (18t \log d) \cdot (\nu + \|\bar{B}\|^2 + m\|\bar{B}\|\epsilon) / (\epsilon^2 \|\bar{B}\|^2) \quad \text{and} \quad \gamma \leq (\epsilon \|\bar{B}\| / (2L))^2$$

792 with probability at least  $1 - 1/d^{2t} - n\gamma$ ,

$$\|\hat{B} - \bar{B}\| \leq \epsilon \|\bar{B}\|.$$

793 **Claim D.7.**  $P_2 = \sum_{i=1}^k v_i m_{j_2,i} (\alpha^\top \bar{w}_i)^{j_2-2} \bar{w}_i^{\otimes 2}$  and  $P_3 = \sum_{i=1}^k v_i m_{j_3,i} (\alpha^\top \bar{w}_i)^{j_3-3} \bar{w}_i^{\otimes 3}$ .
