# Supplementary material for: Going Beyond Linear RL: Sample Efficient Neural Function Approximation
Source: arXiv:2107.06466 source file (2021-12-25)
Supplement: Supplementary file 3 [file additional_prelim.tex]

\section{Additional Preliminaries}
