# Supplementary material for: Going Beyond Linear RL: Sample Efficient Neural Function Approximation
Source: arXiv:2107.06466 source file (2021-12-25)
Supplement: Supplementary file 4 [file proof_.tex]

\section{Proofs for $\cdots$}
